# Supplementary material for: Spatio-temporal Symmetry - Point Groups with Time Translations
Source: arXiv:1701.04088 ancillary file (2017-09-21)

# Spatio-temporal Symmetry - Point Groups with Time Translations

## Supplementary Information - Stereographic Projections

Haricharan Padmanabhan, Maggie L. Kingsland, Jason M. Munro,
Daniel B. Litvin, and Venkatraman Gopalan

The stereographic projections of point groups with time-translations are listed below, ordered by serial number as defined in the main text. Time translations are indicated in the diagram in a manner similar to how spatial translations perpendicular to the plane are indicated in space-group diagrams. Non-zero time translations are visually indicated by numbers in blue. No number implies a time translation of zero. The spatial element associated with a time translation is identified within the plane by proximity, and out of the plane using the superscript. Each figure has the spatio-temporal group index on the top-left, the normal subgroup of the spatio-temporal group with vanishing time translations on the top-center, and the corresponding point group on the top-right.

Anticlockwise is positive for axial rotations in all figures. For the point groups with three-fold and six-fold axial symmetry, the following convention is used - the axis '1' is chosen to be along the in-plane horizontal direction, and the axis 'x' makes an angle of $-\pi/6$ with respect to it. The sets of axes 1, 2, and 3, and x, y, and xy are each generated by threefold rotations about the out-of-plane direction.

**1.1.1** **1** **1**

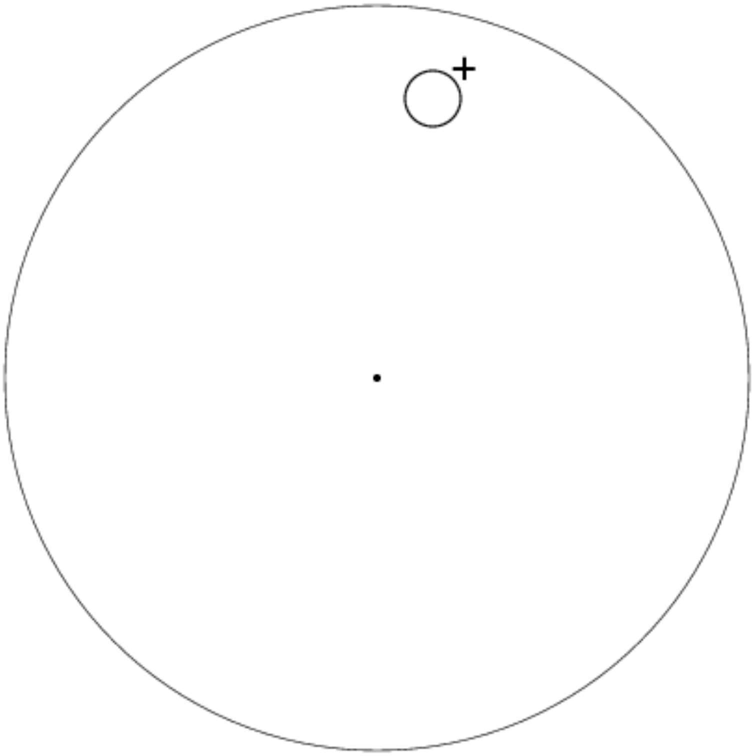

**2.1.2** $\bar{1}$ $\bar{1}$

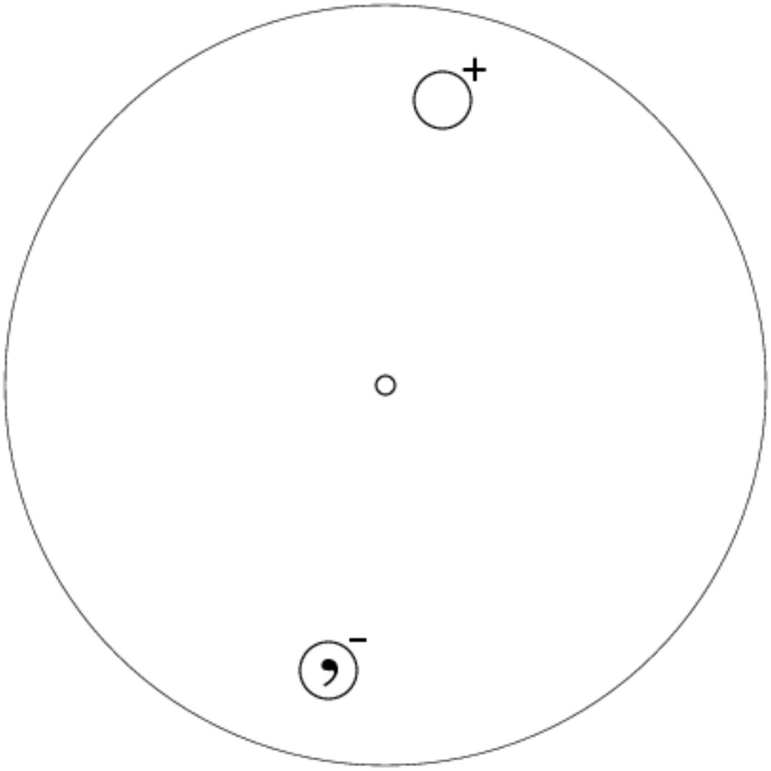

**2.2.3** **1** **$\bar{1}$**

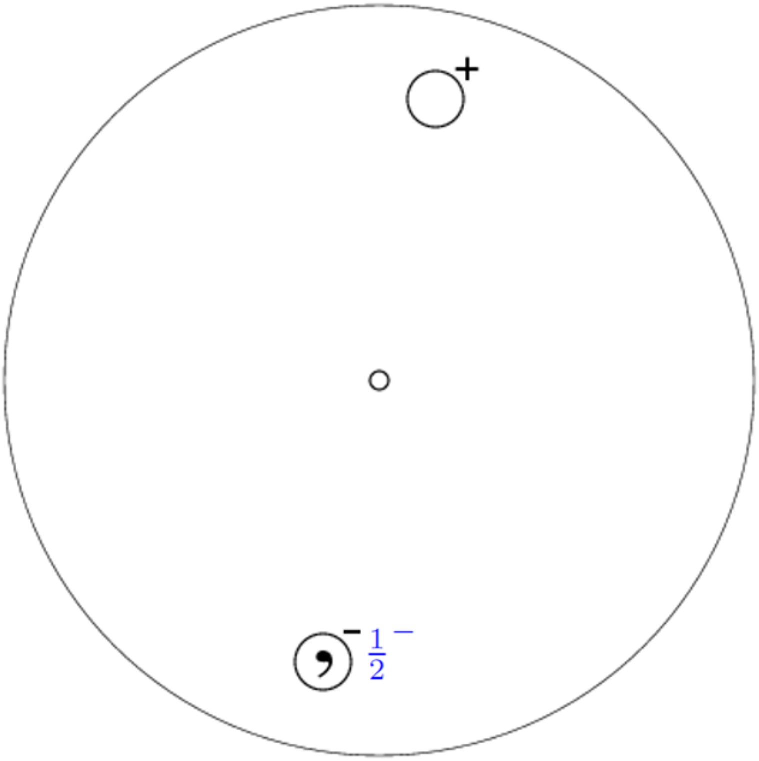

**3.1.4** **2** **2**

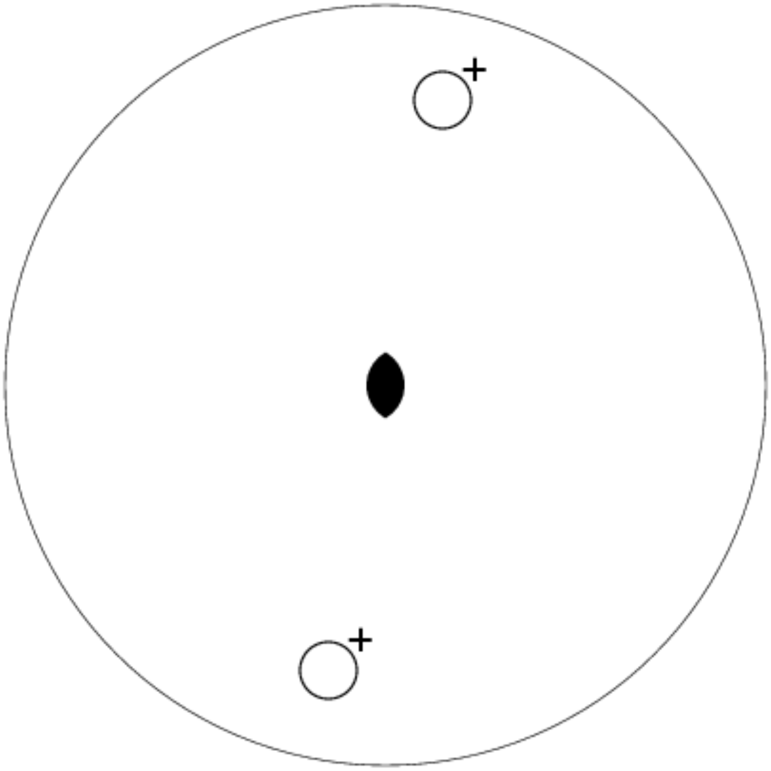

**3.2.5 1 2**

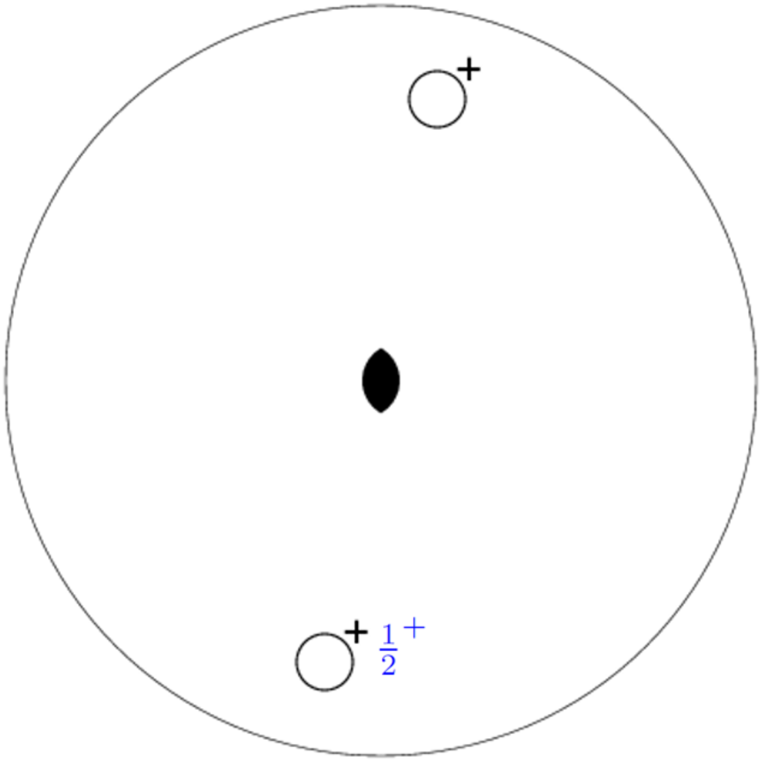

**4.1.6** **m** **m**

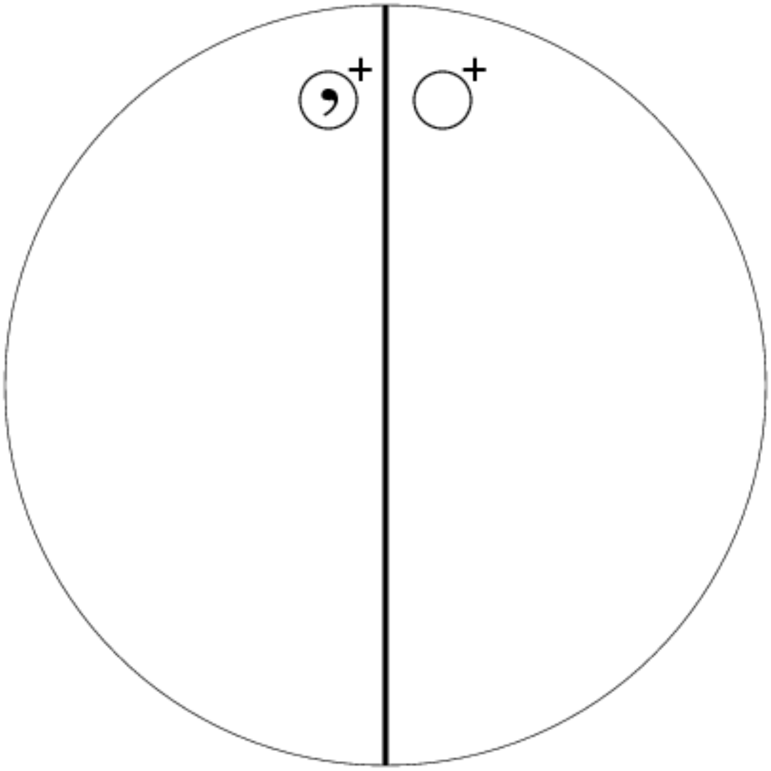

**4.2.7** **1** **m**

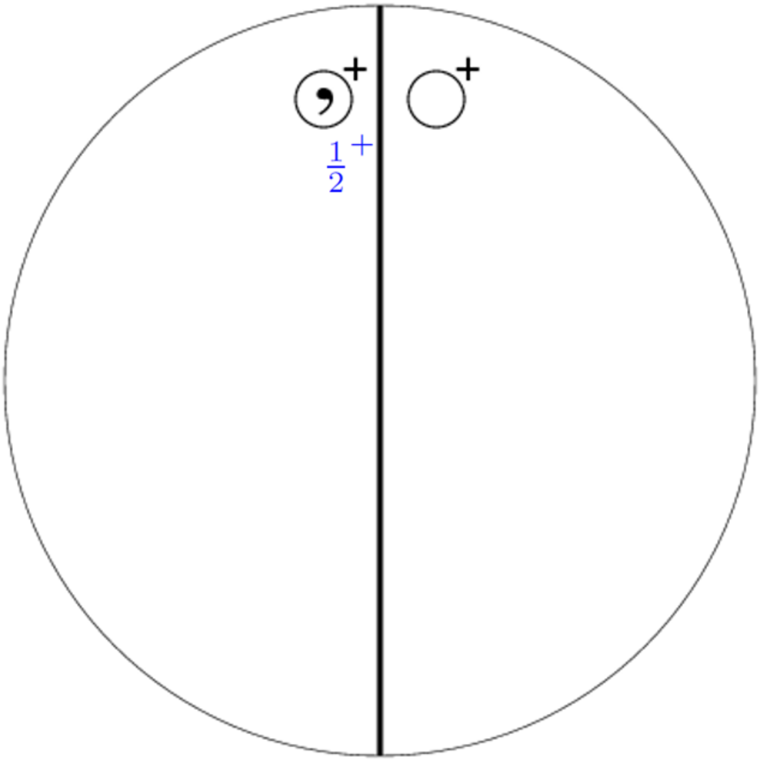

**5.1.8** **2/m** **2/m**

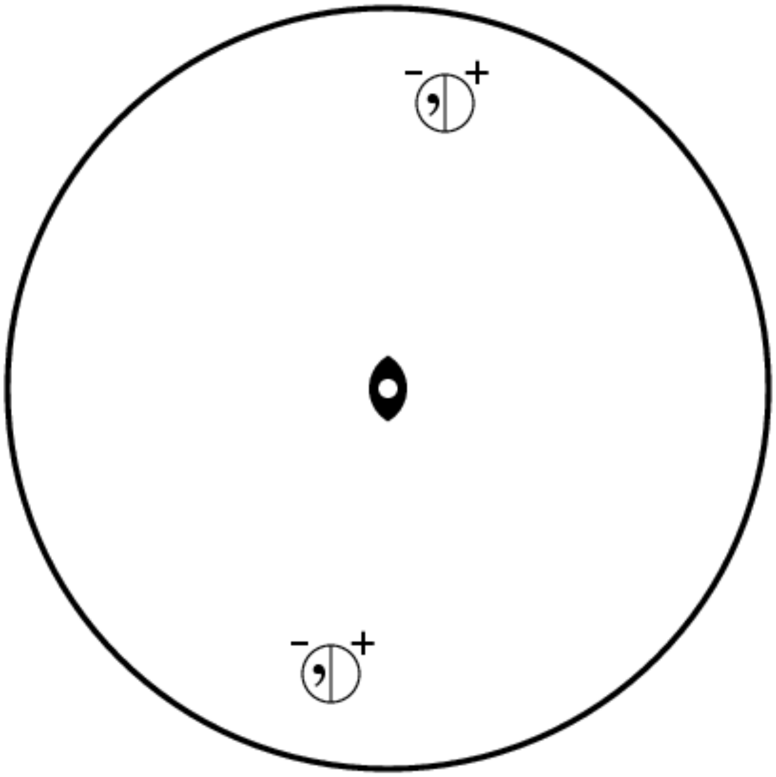

**5.2.9** **$\bar{1}$** **2/m**

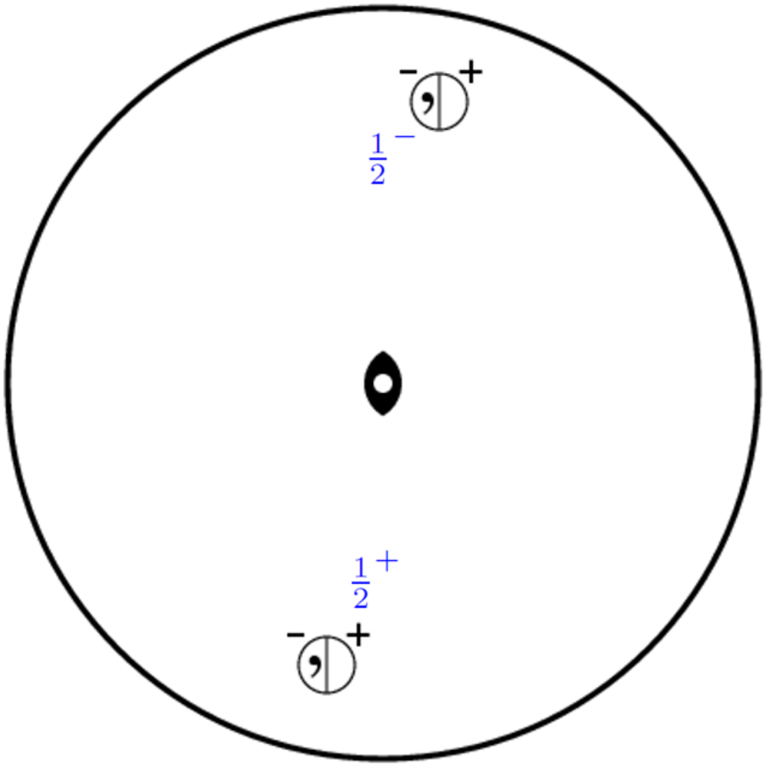

**5.3.10** **2** **2/m**

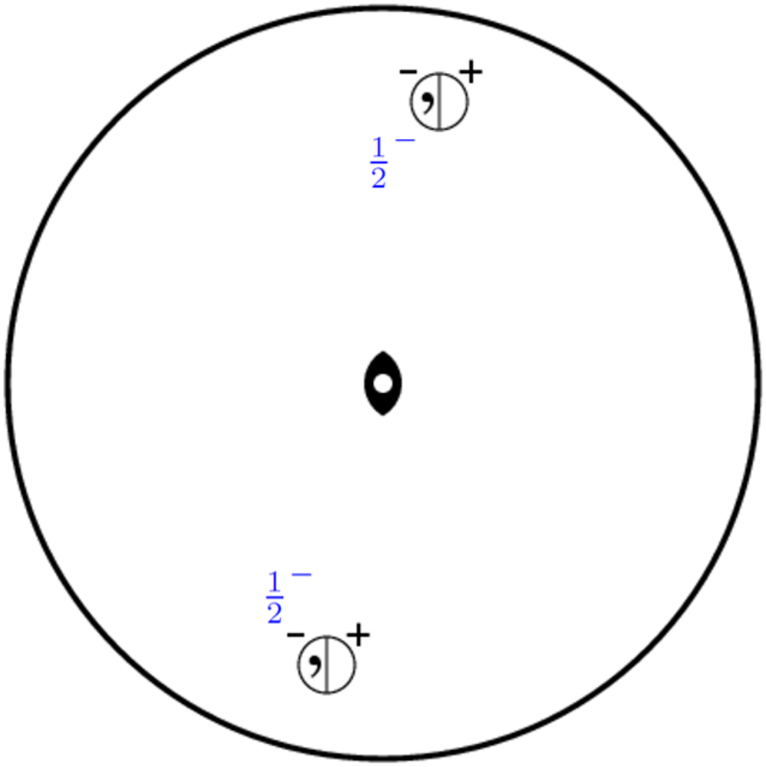

**5.4.11** **1** **2/m**

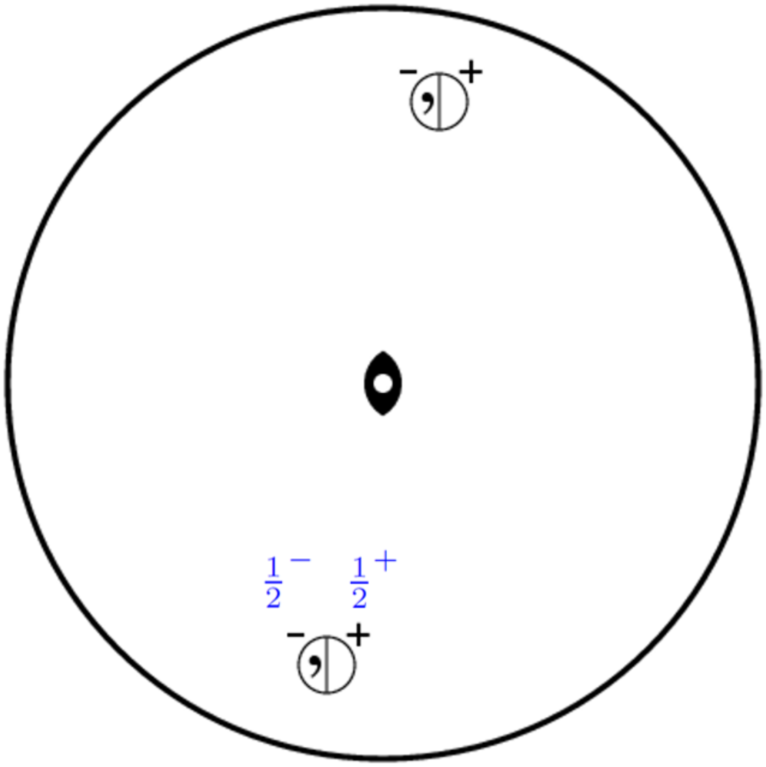

**6.1.12** **222** **222**

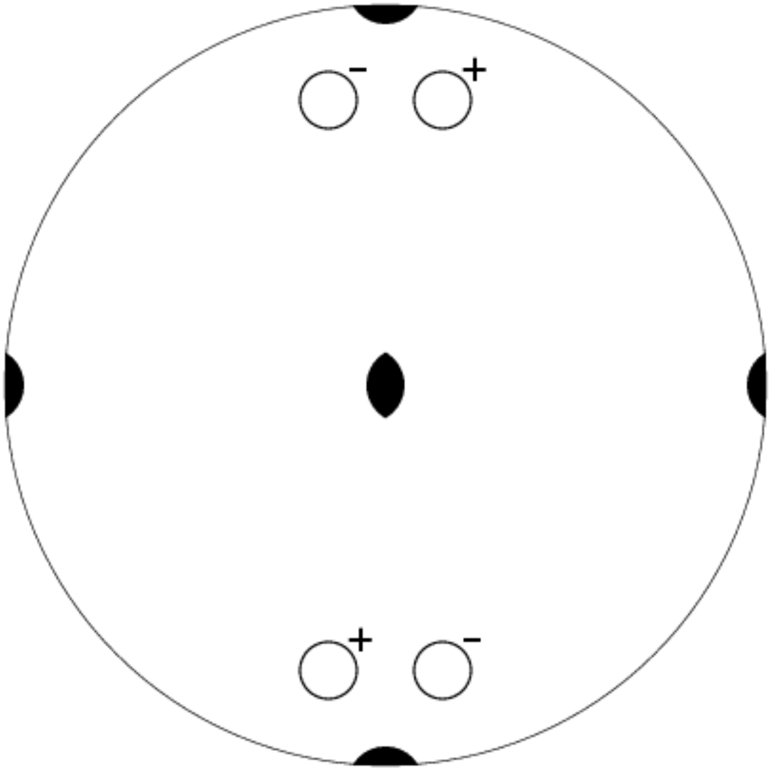

**6.2.13** **2** **222**

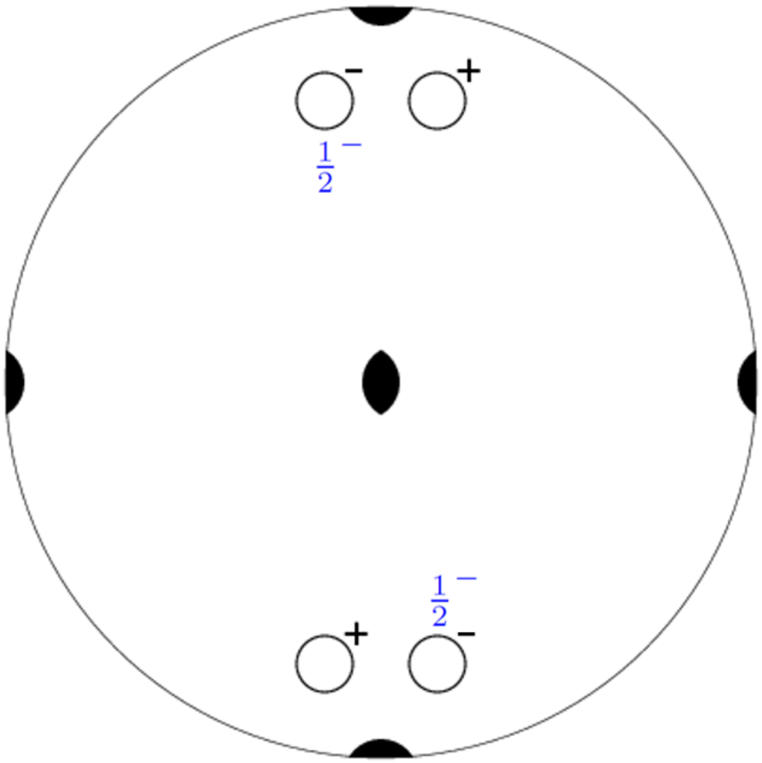

**7.1.14** **mm2** **mm2**

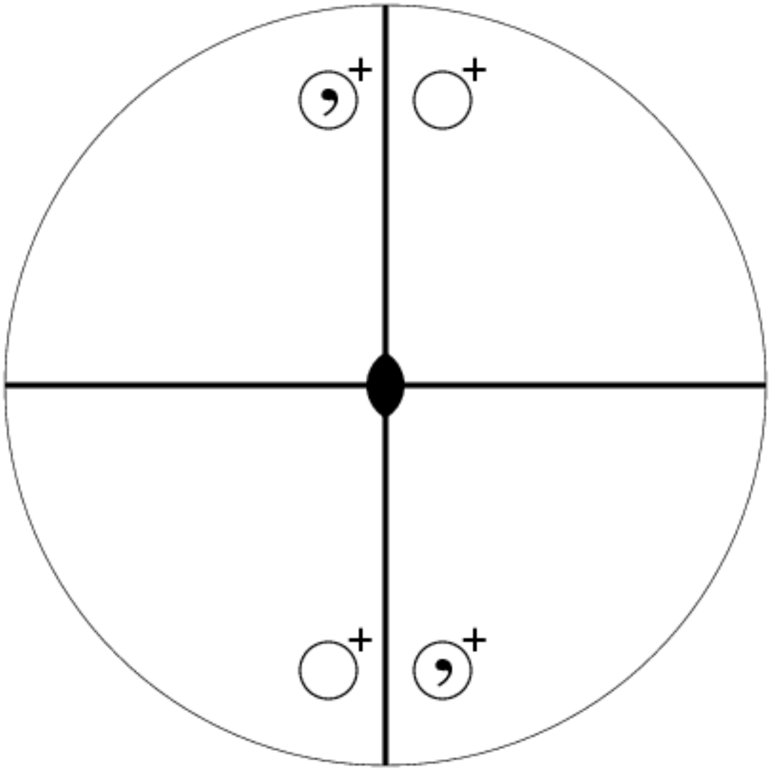

**7.2.15** **2** **mm2**

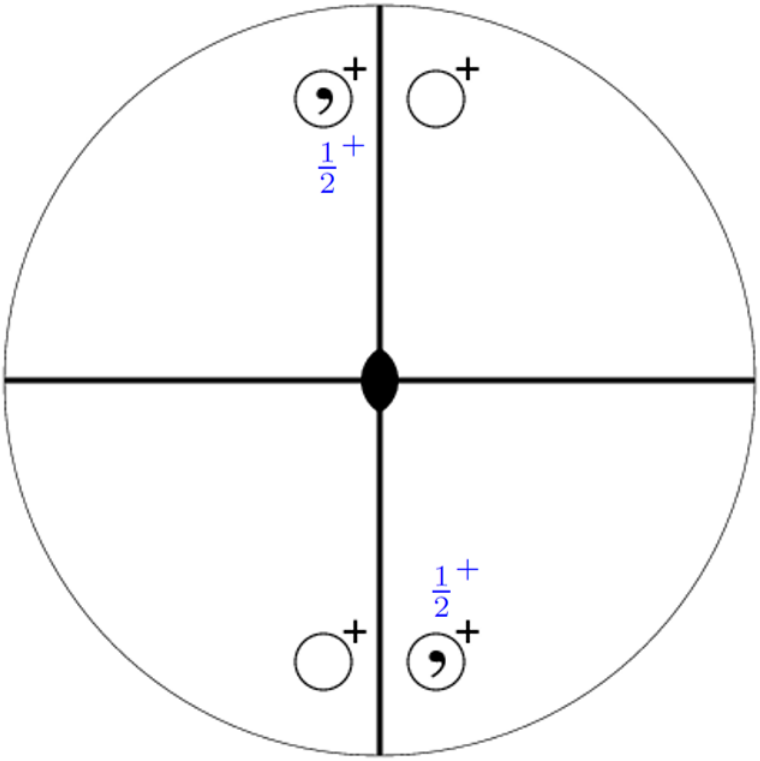

**7.3.16** **m** **mm2**

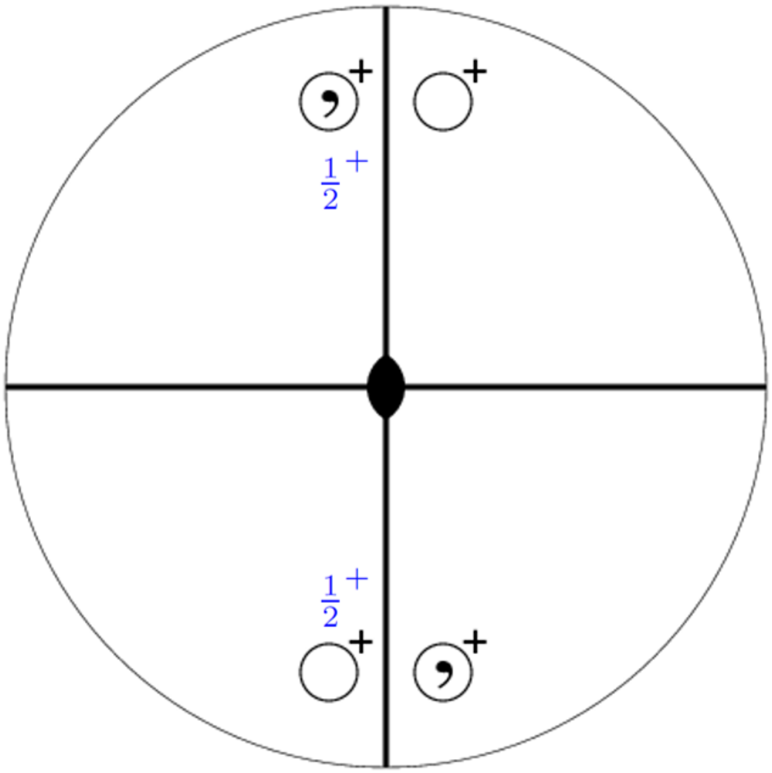

**8.1.17** **mmm** **mmm**

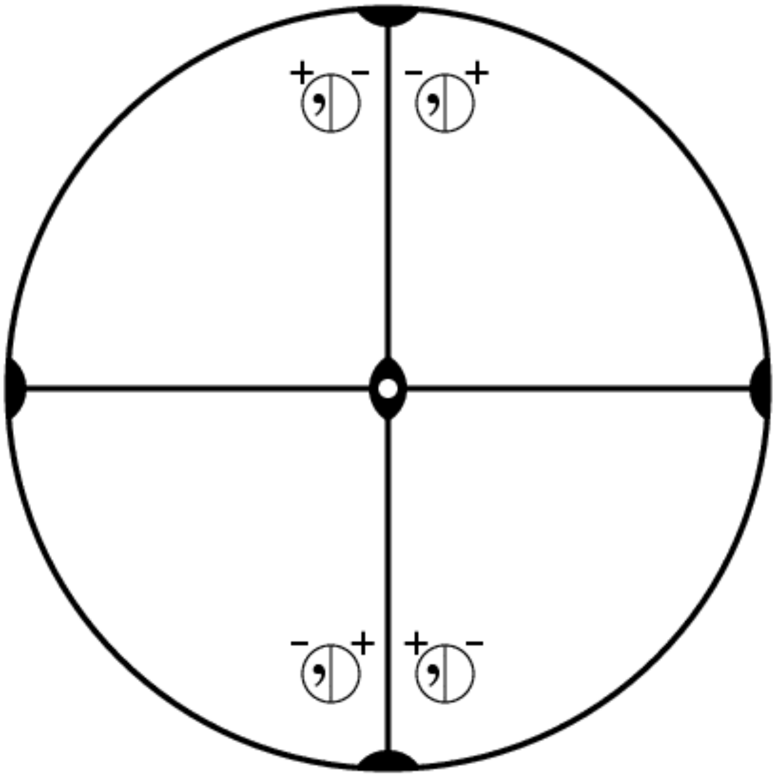

**8.2.18** **2/m** **mmm**

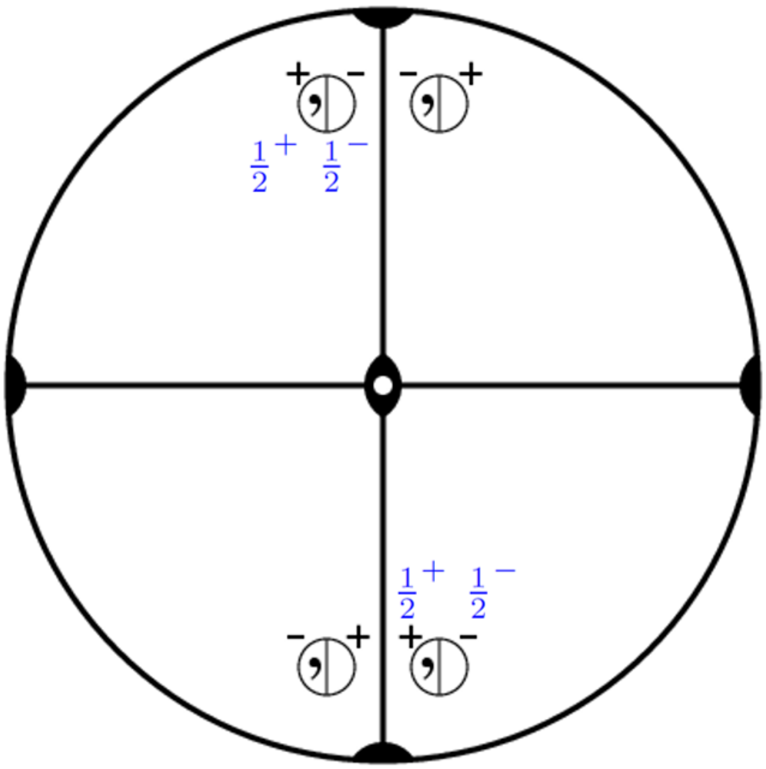

**8.3.19** **222** **mmm**

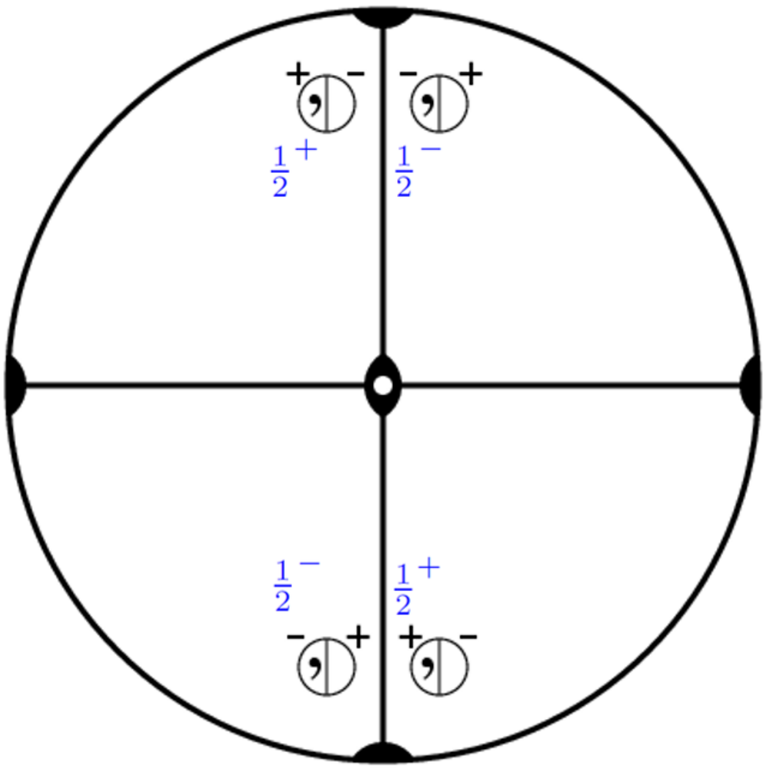

**8.4.20** **mm2** **mmm**

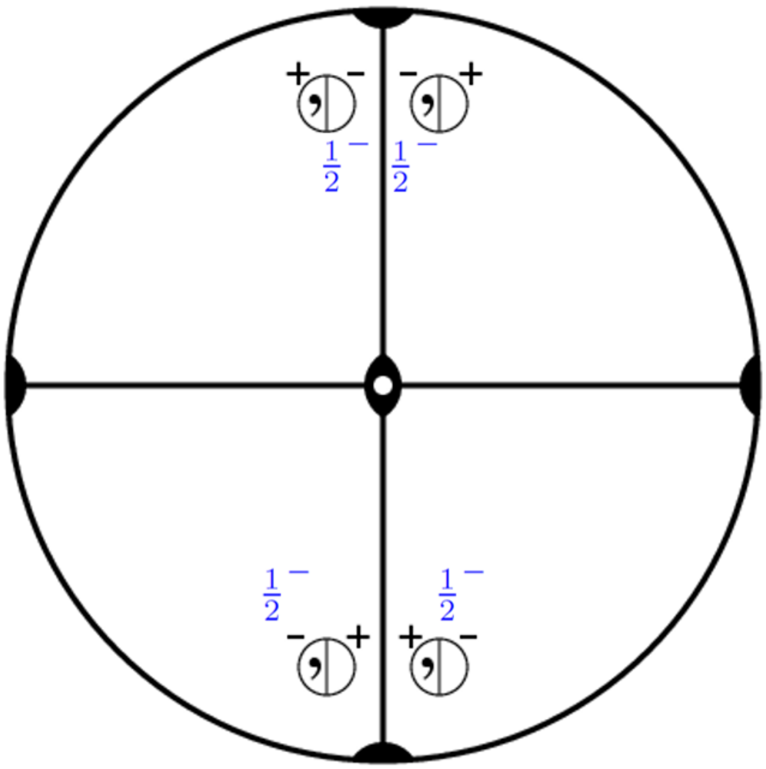

**9.1.21** **4** **4**

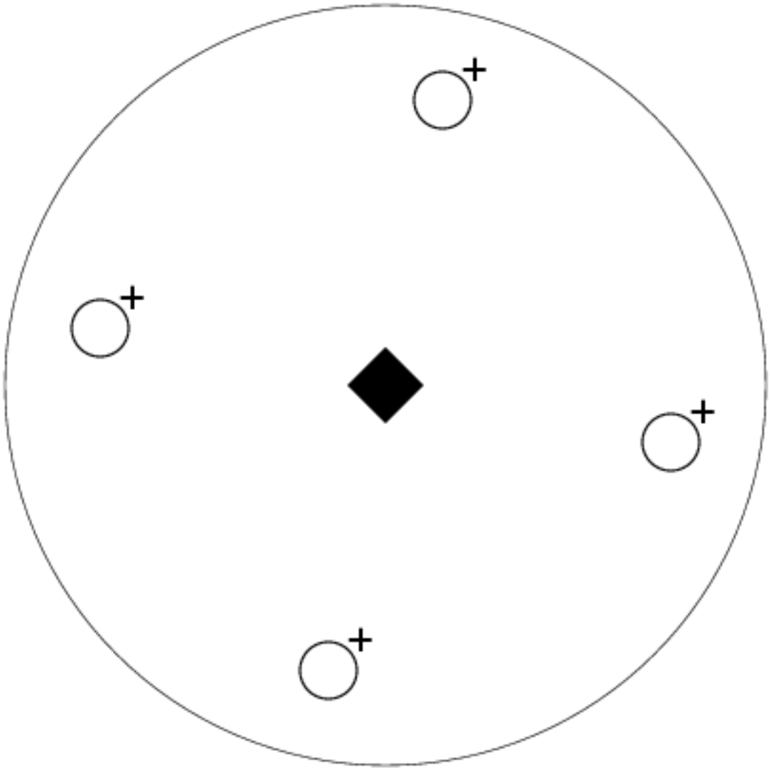

**9.2.22** **2** **4**

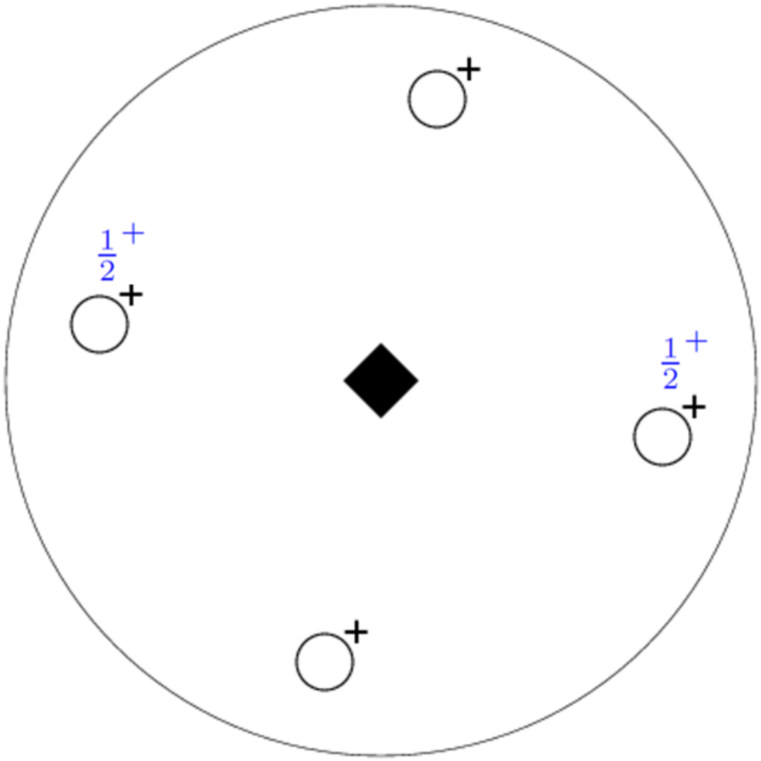

**9.3.23** **1** **4**

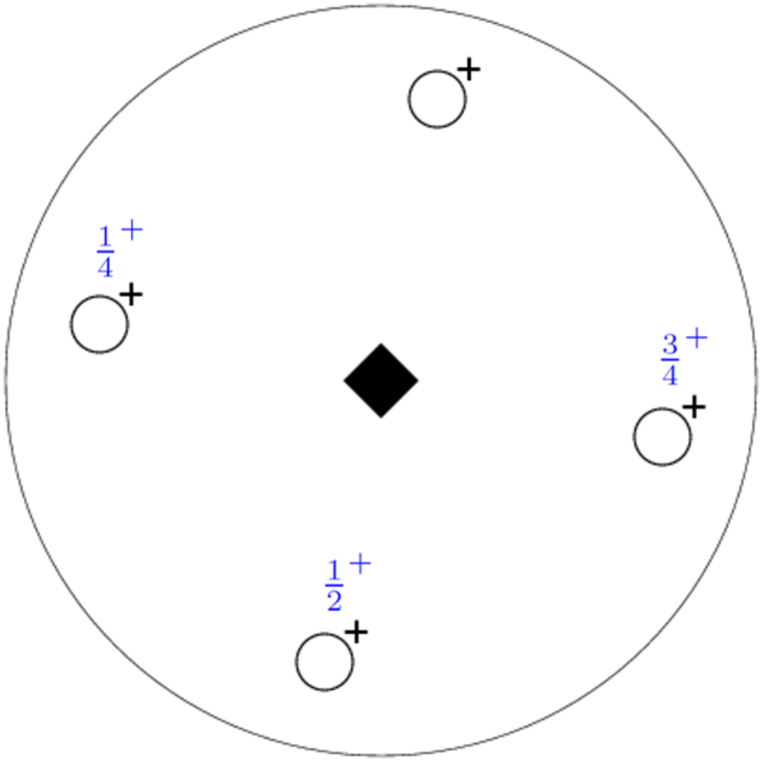

**10.1.24** **$\bar{4}$** $\bar{4}$

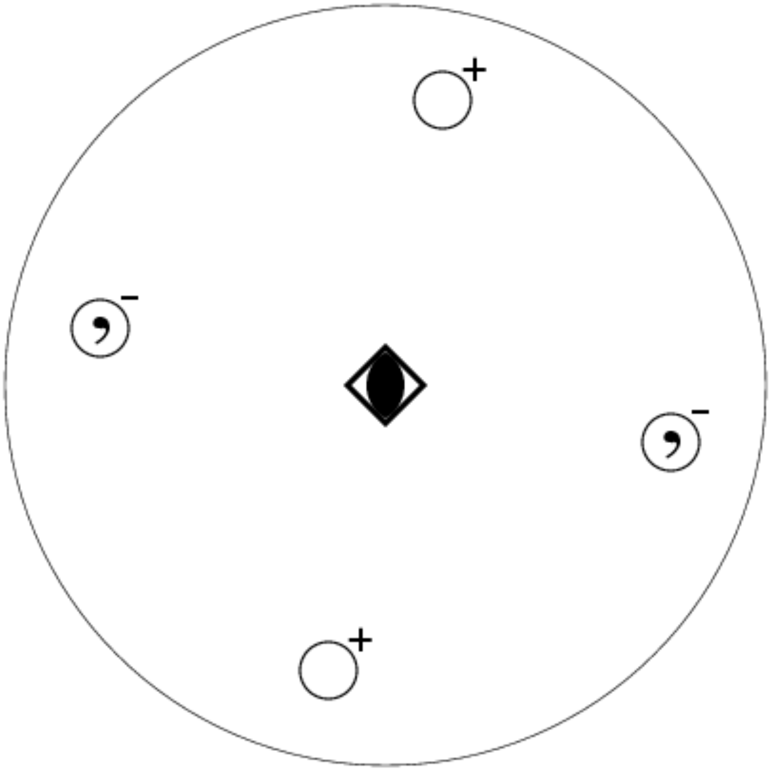

**10.2.25** **2** $\bar{4}$

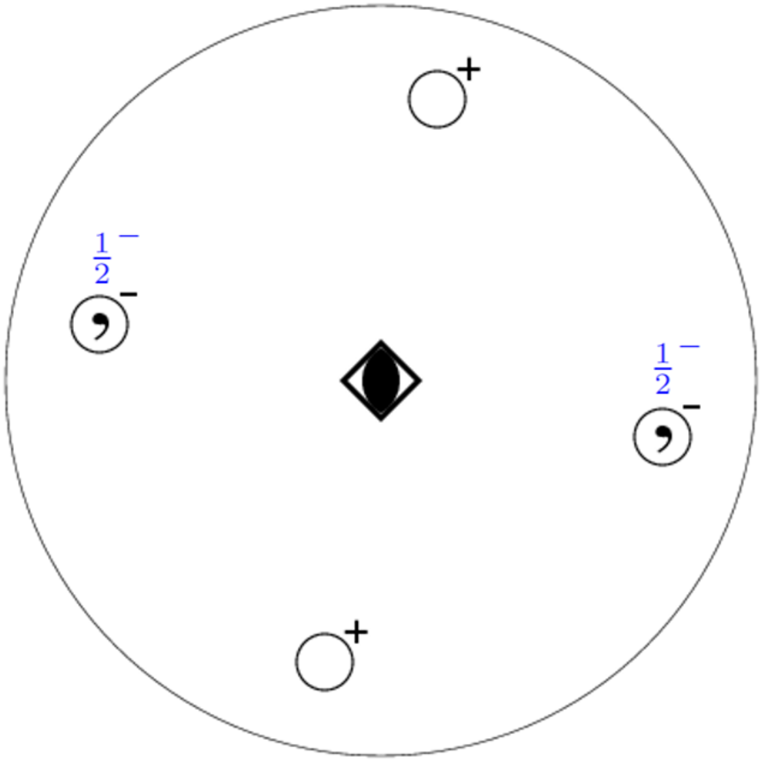

**10.3.26** **1** $\bar{4}$

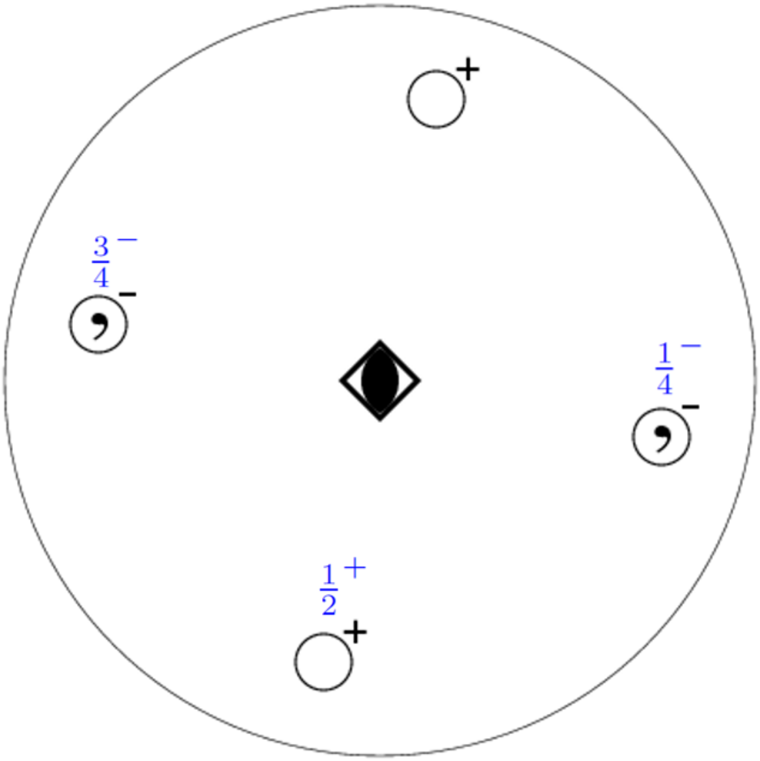

**11.1.27** **4/m** **4/m**

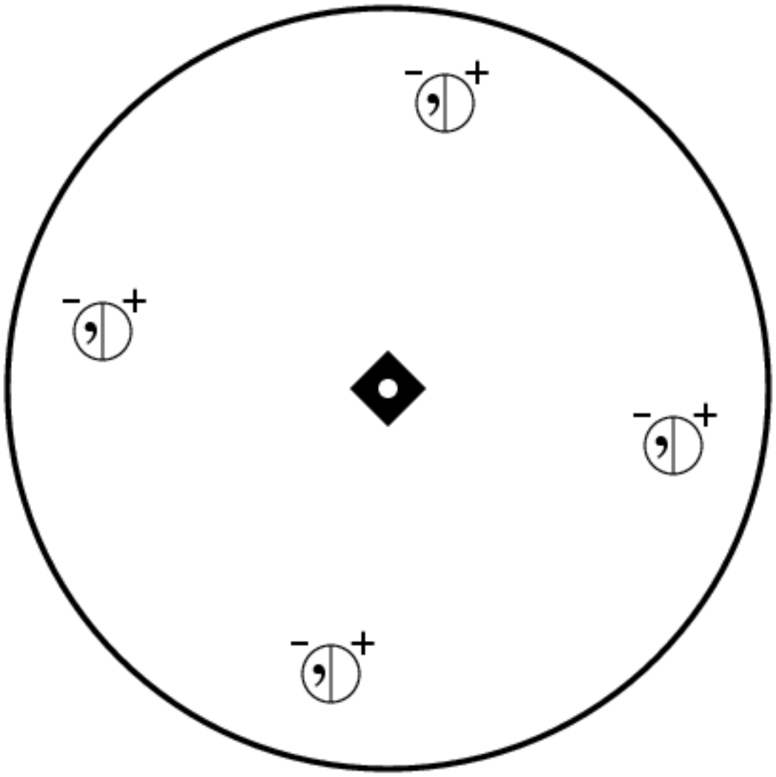

**11.2.28** **2/m** **4/m**

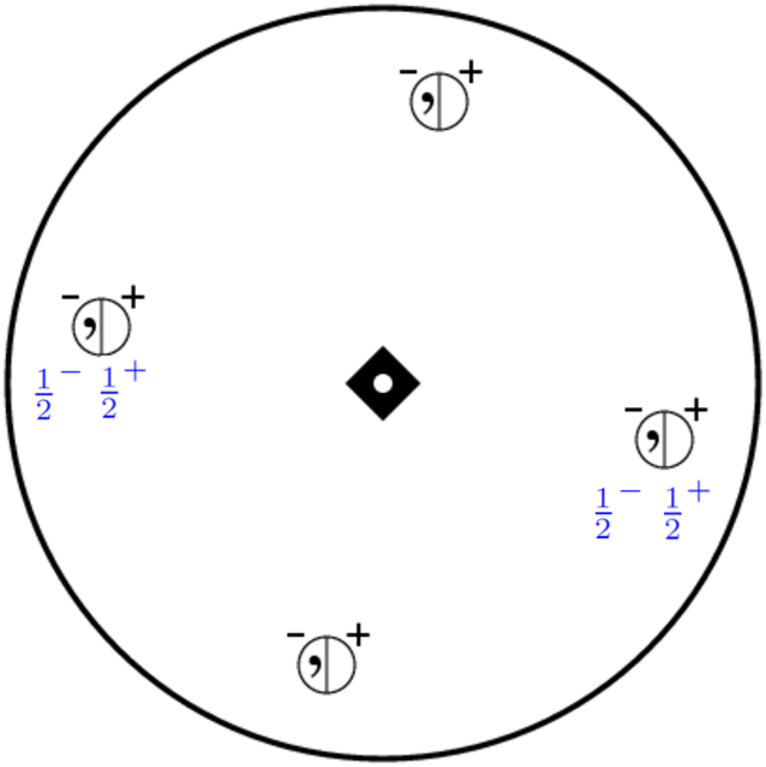

**11.3.29** **$\bar{1}$** **4/m**

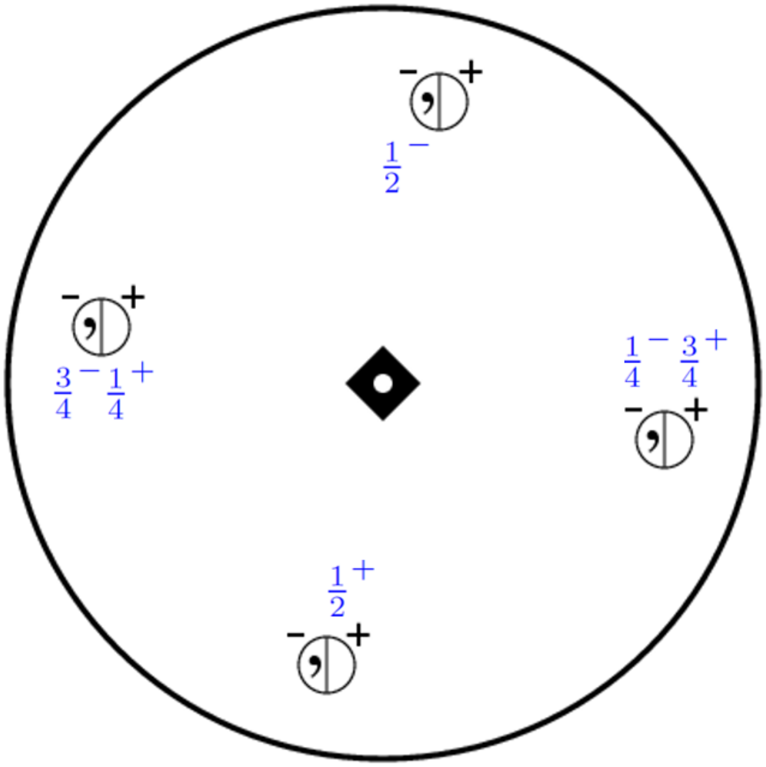

**11.4.30** **4** **4/m**

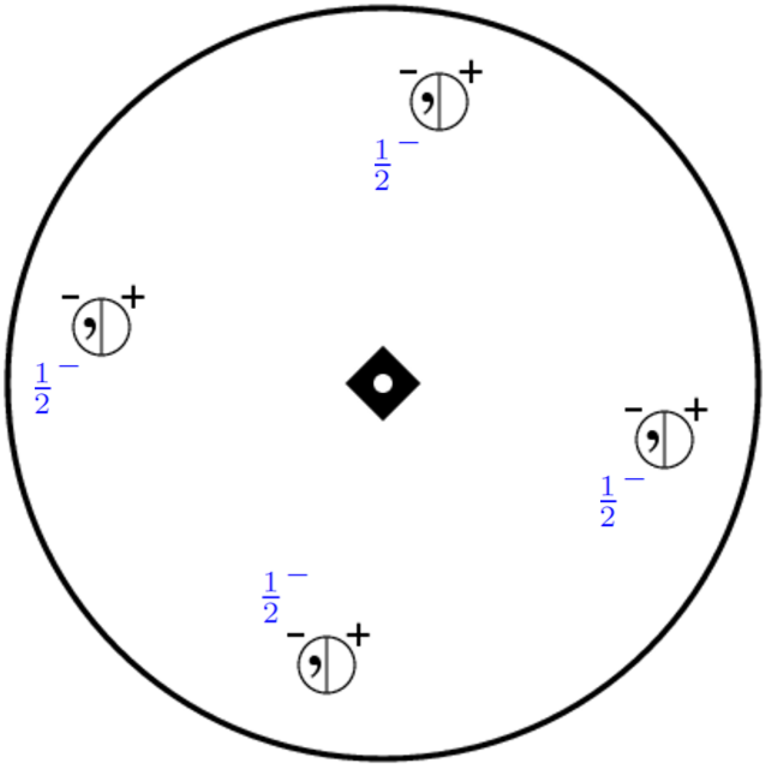

**11.5.31** **$\bar{4}$** **4/m**

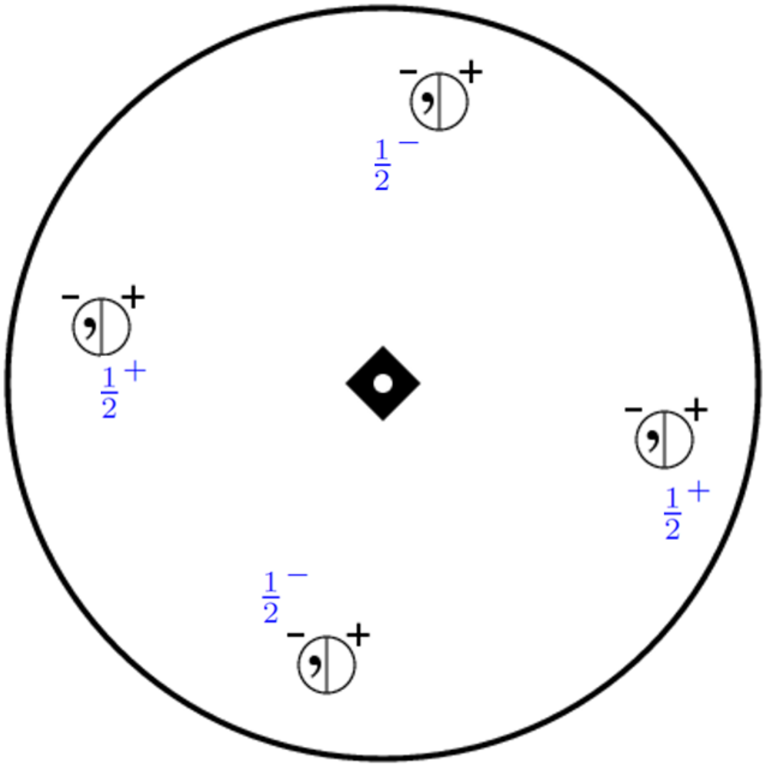

**11.6.32** **m** **4/m**

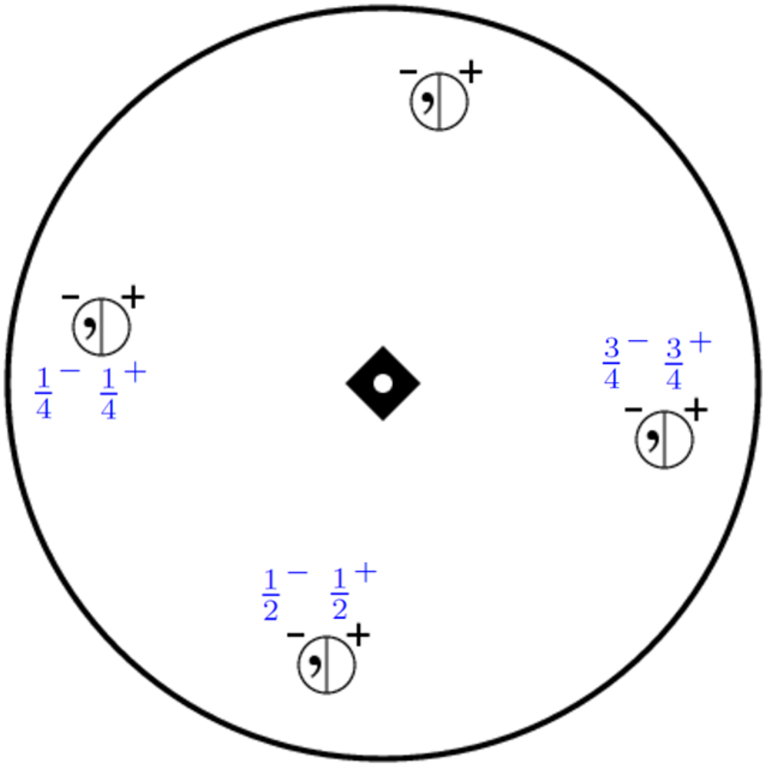

**12.1.33** **422** **422**

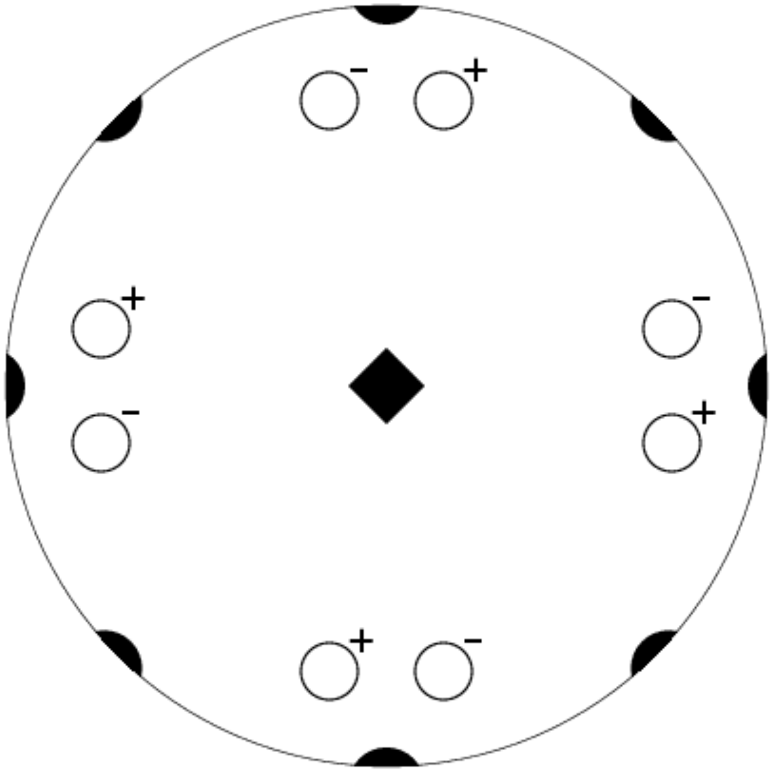

**12.2.34** **4** **422**

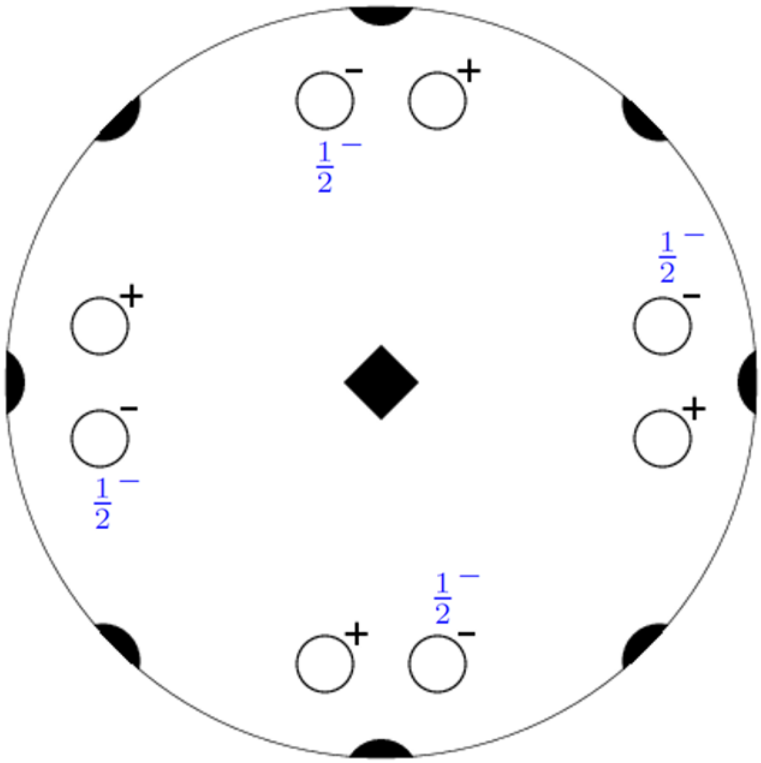

**12.3.35** **222** **422**

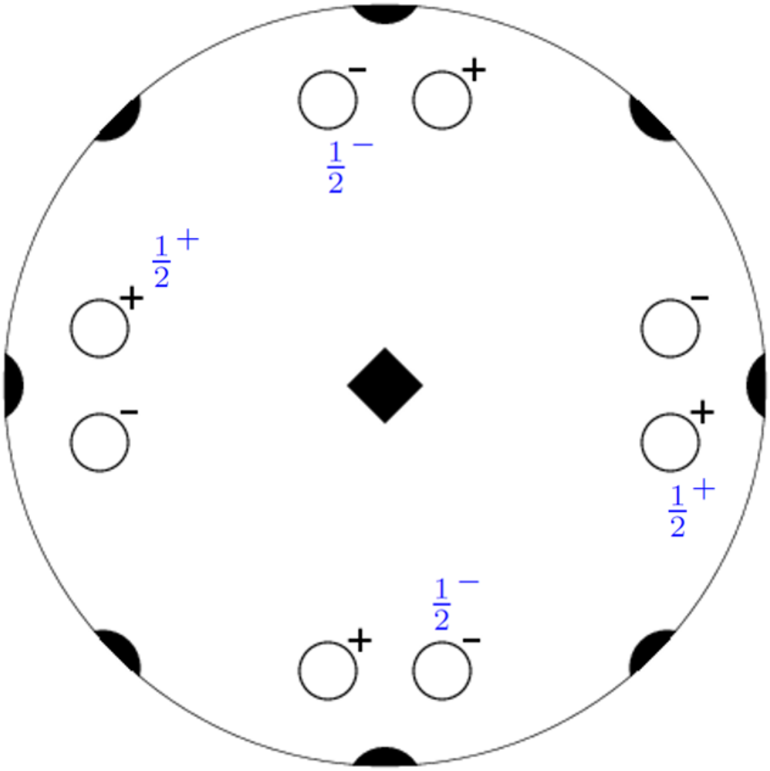

**13.1.36** **4mm** **4mm**

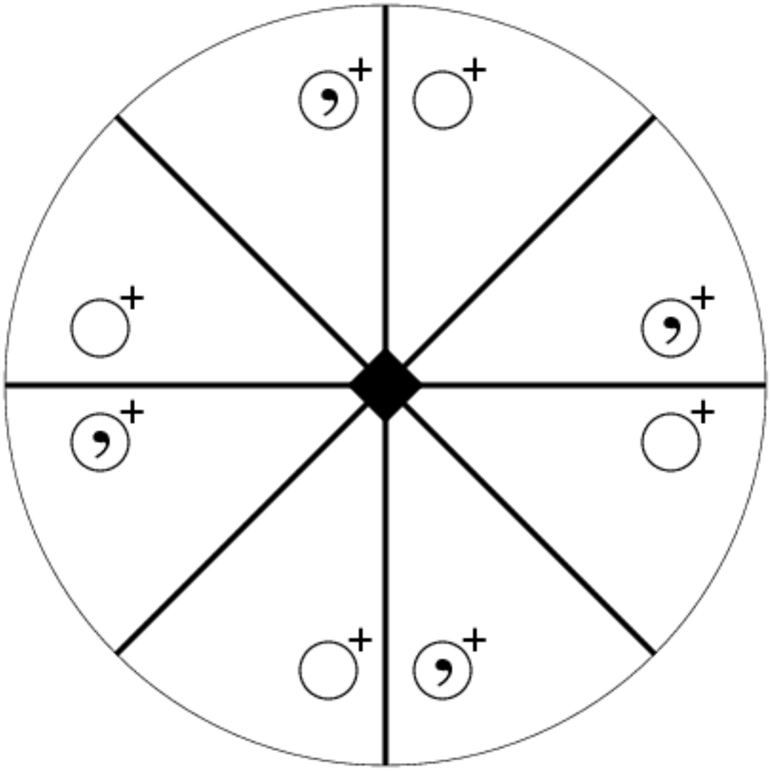

**13.2.37** **4** **4mm**

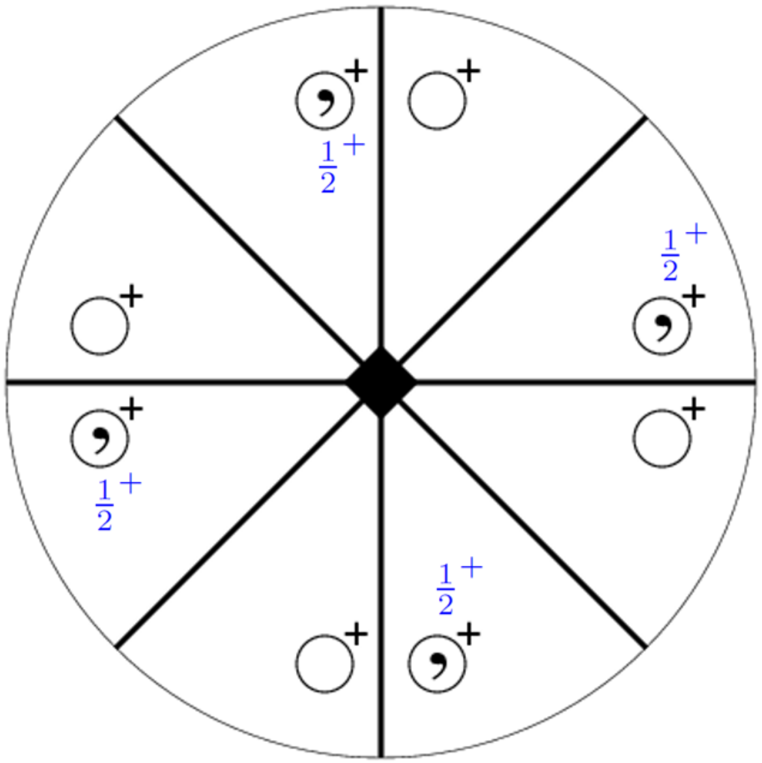

**13.3.38** **mm2** **4mm**

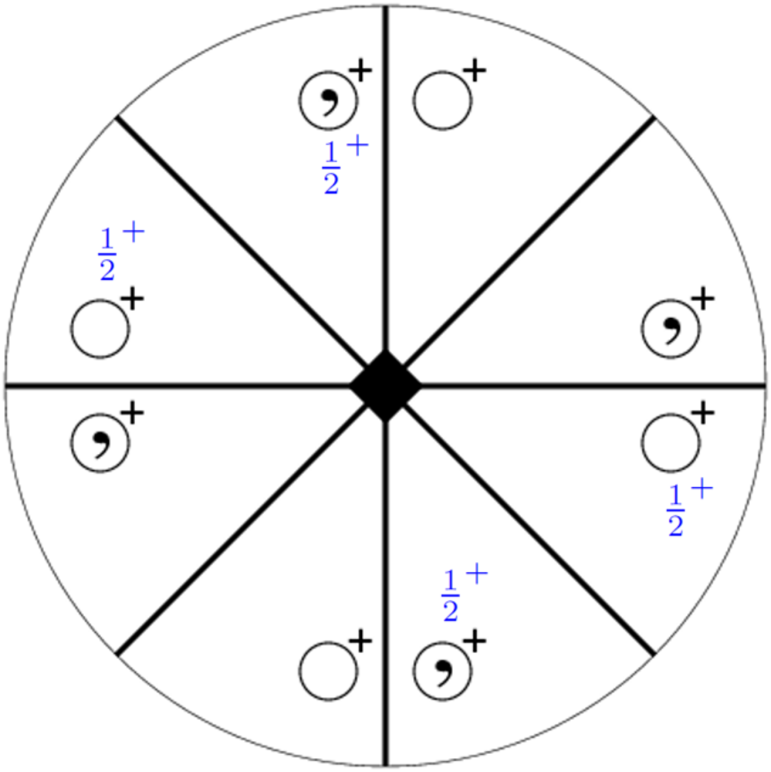

**14.1.39** **$\bar{4}$2m** $\bar{4}$2m

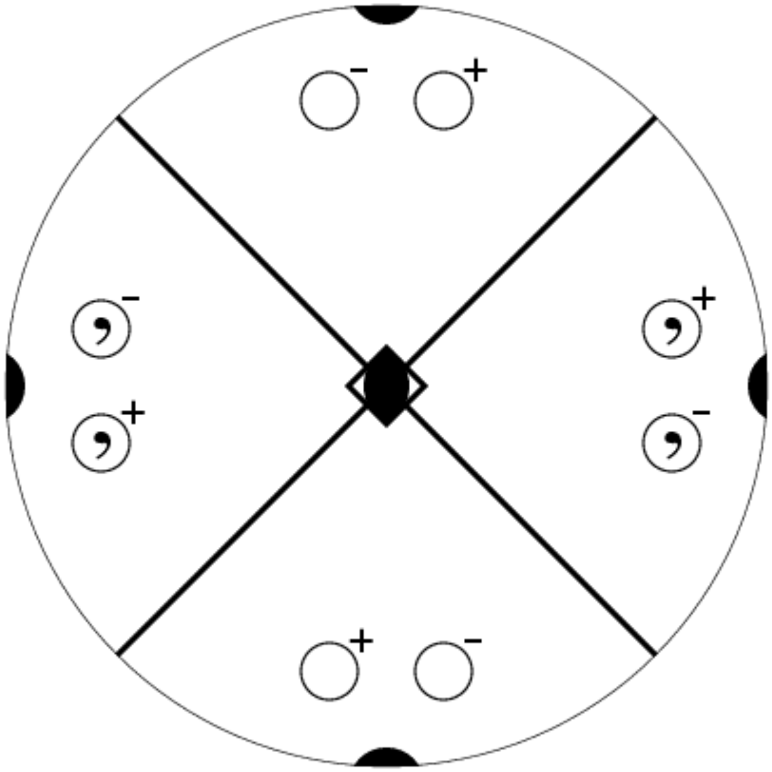

**14.2.40** **$\bar{4}$** **$\bar{4}$2m**

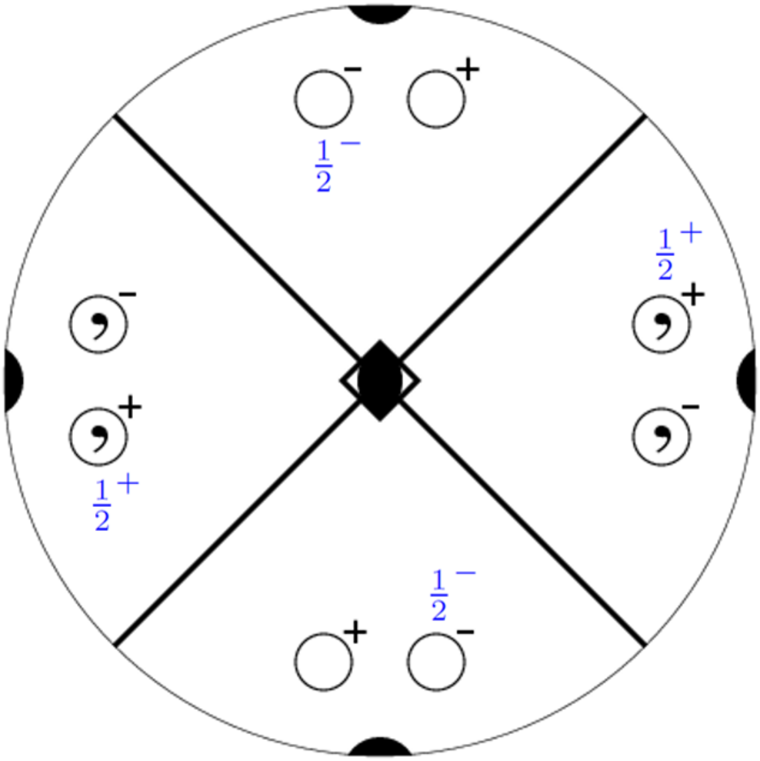

**14.3.41** **222** **$\bar{4}$2m**

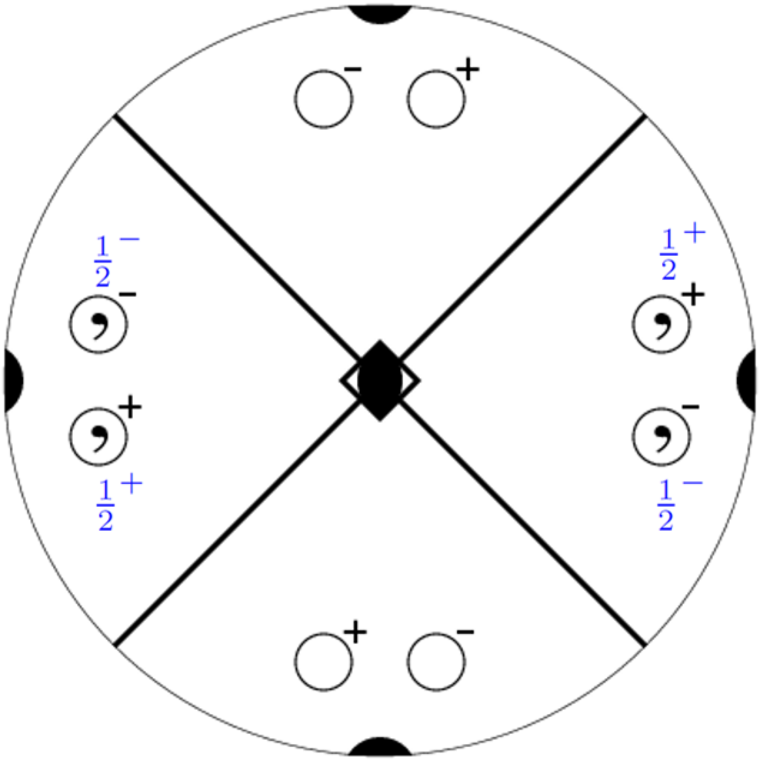

**14.4.42** **mm2** **$\bar{4}$2m**

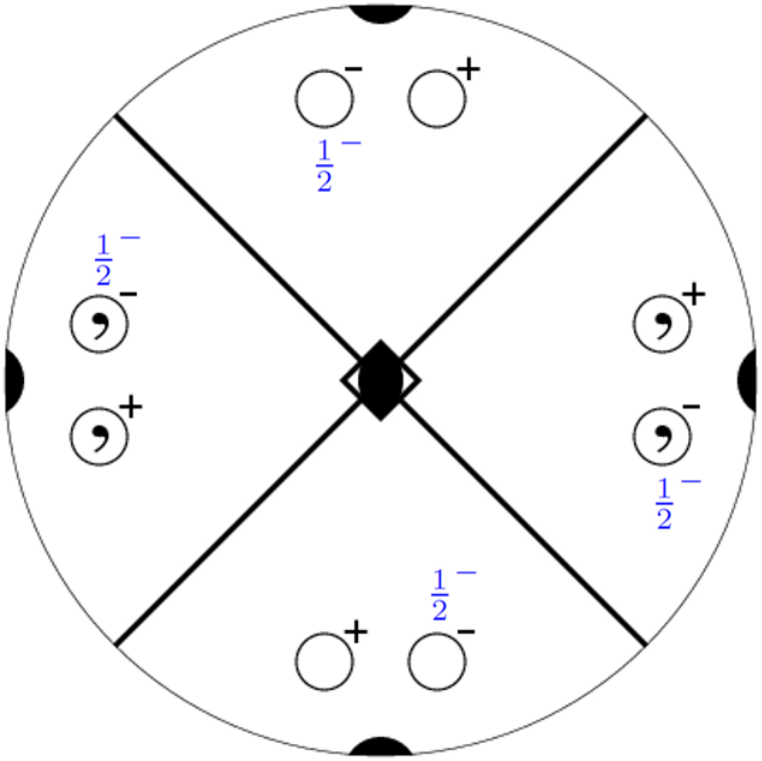

**15.1.43** **4/mmm** **4/mmm**

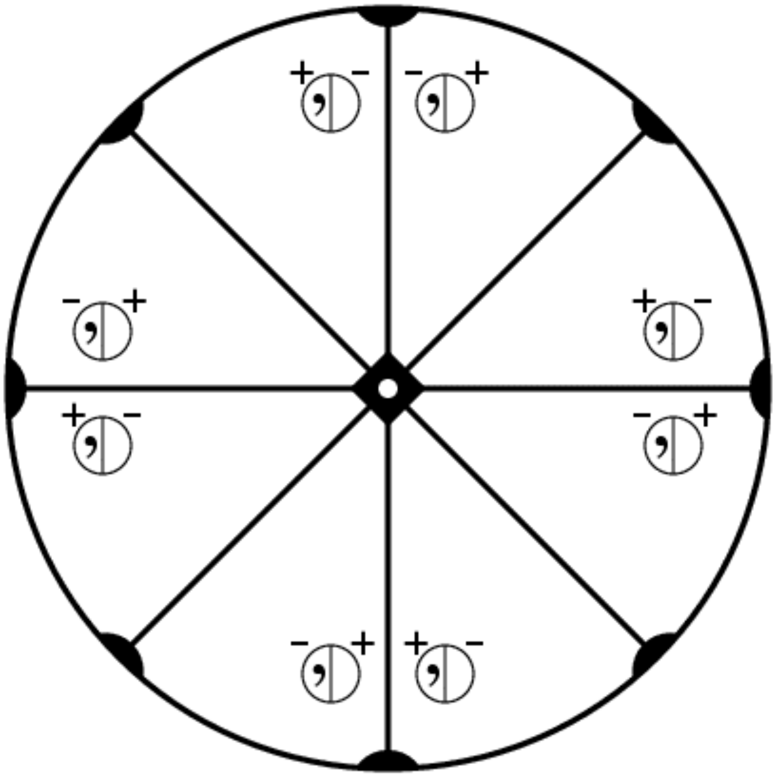

**15.2.44** **$\bar{4}$** **4/mmm**

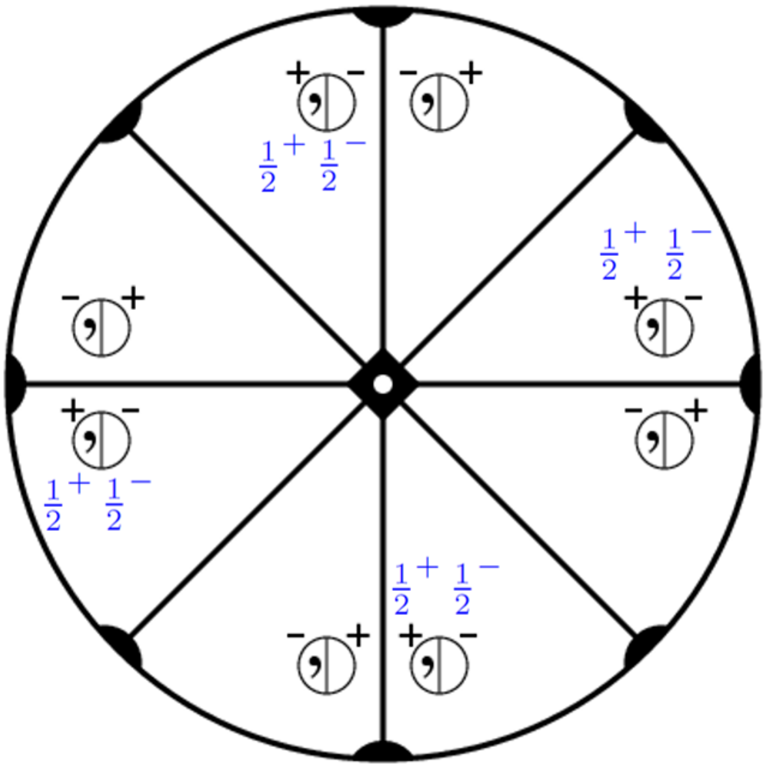

**15.3.45** **mmm** **4/mmm**

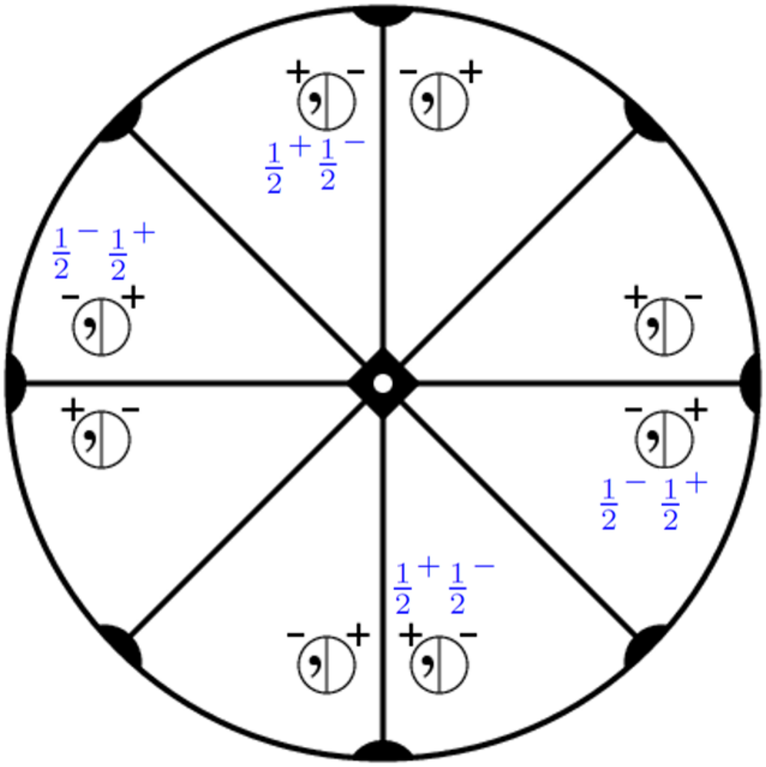

**15.4.46** **422** **4/mmm**

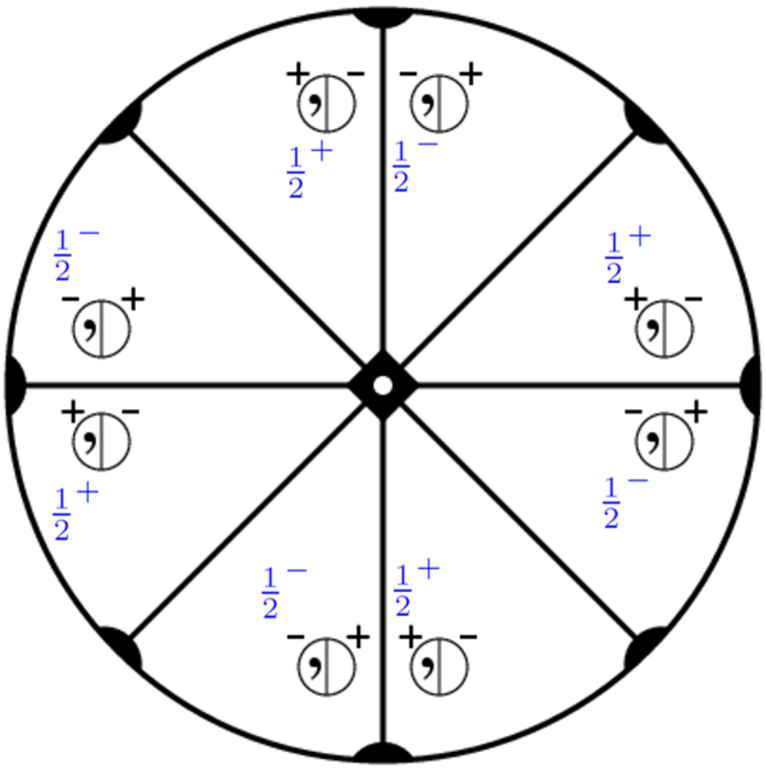

**15.5.47** **4mm** **4/mmm**

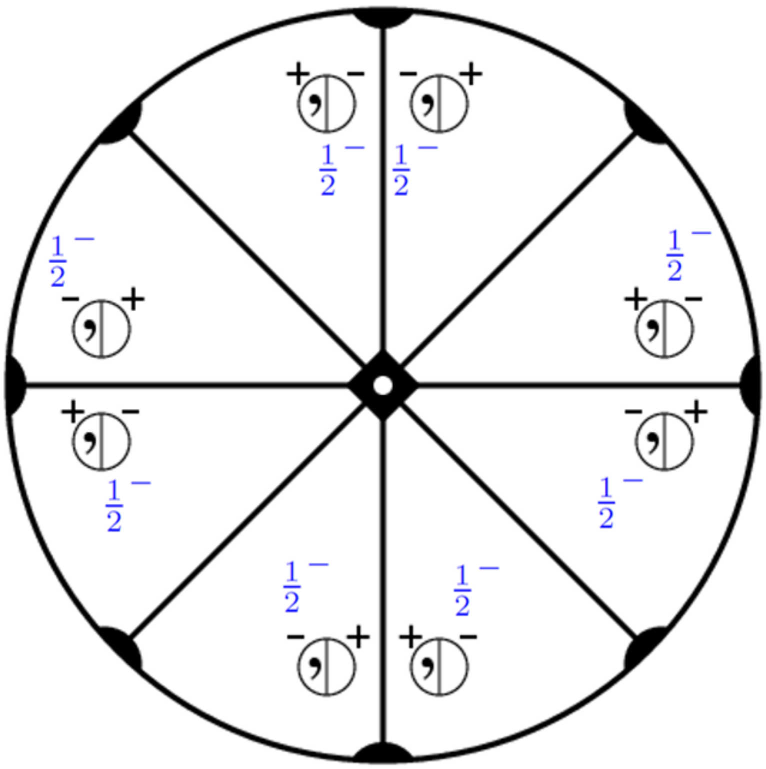

**15.6.48** **$\bar{4}2m$** **4/mmm**

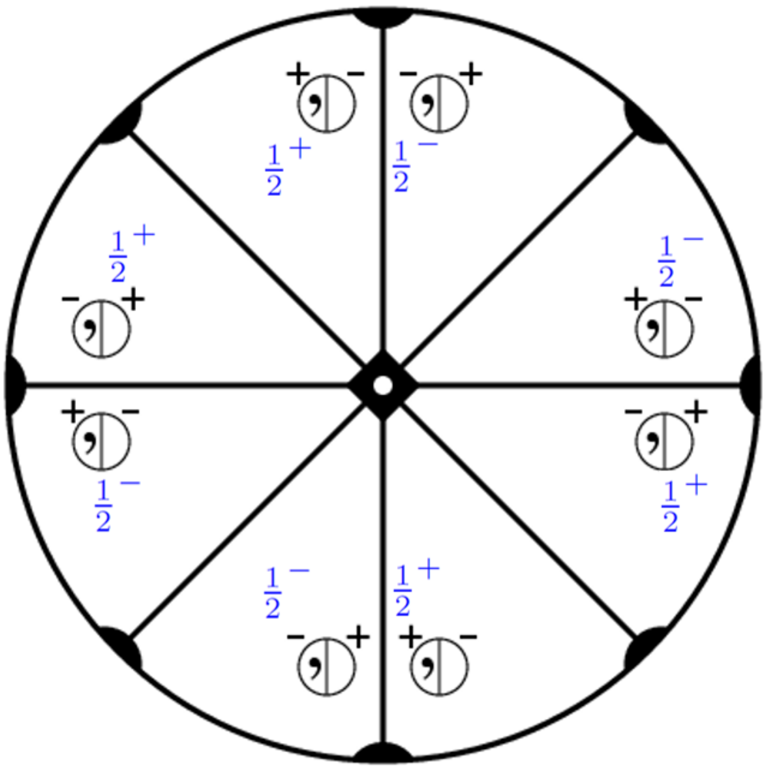

**16.1.49** **3** **3**

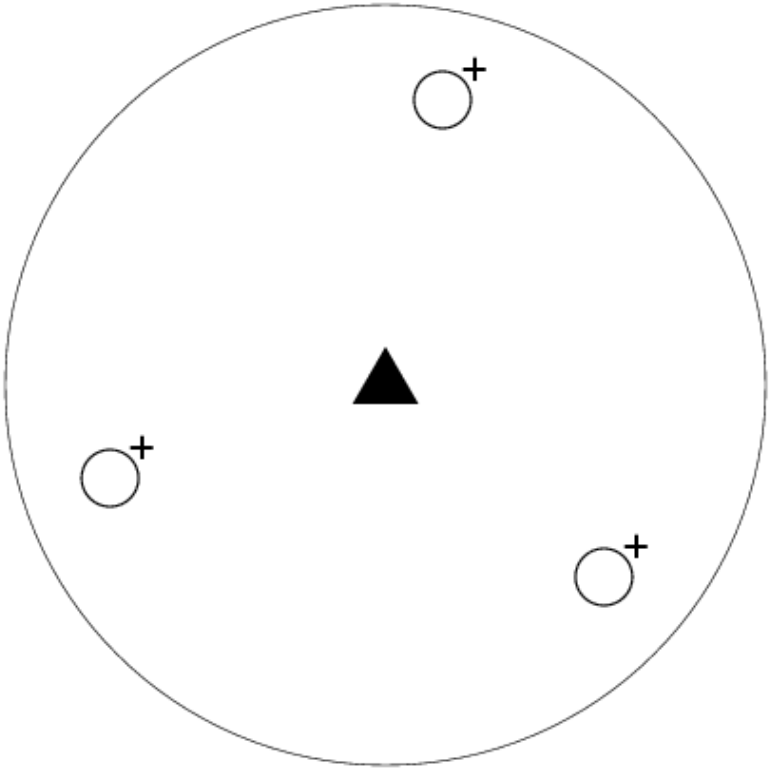

**16.2.50** **1** **3**

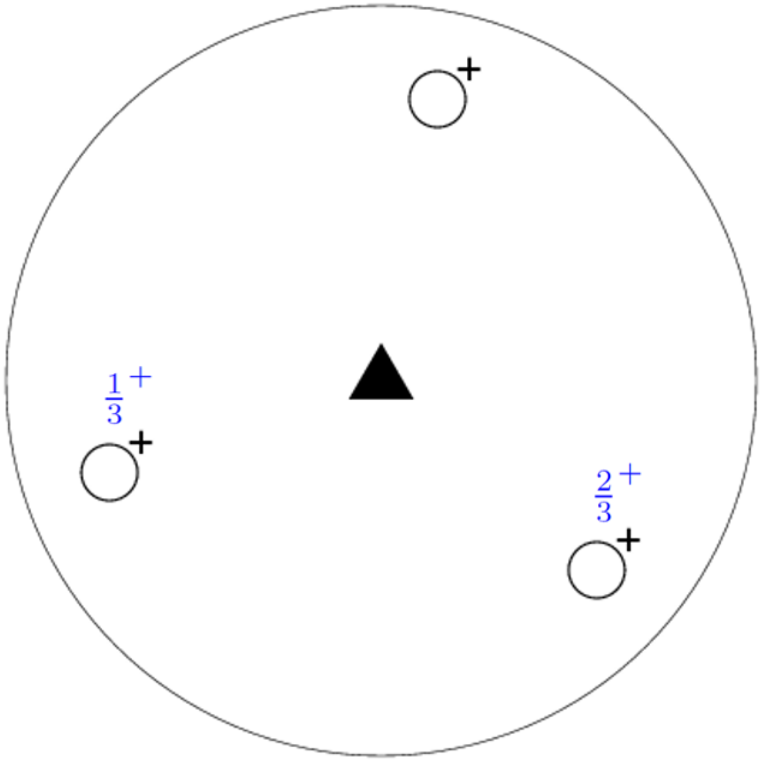

**17.1.51** **$\bar{3}$** $\bar{3}$

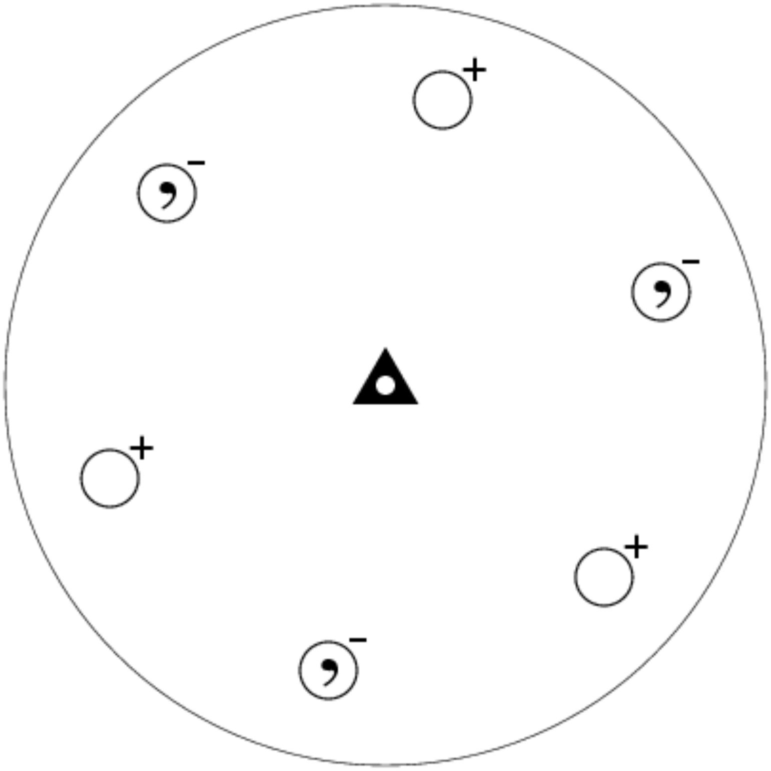

**17.2.52** $\bar{1}$ $\bar{3}$

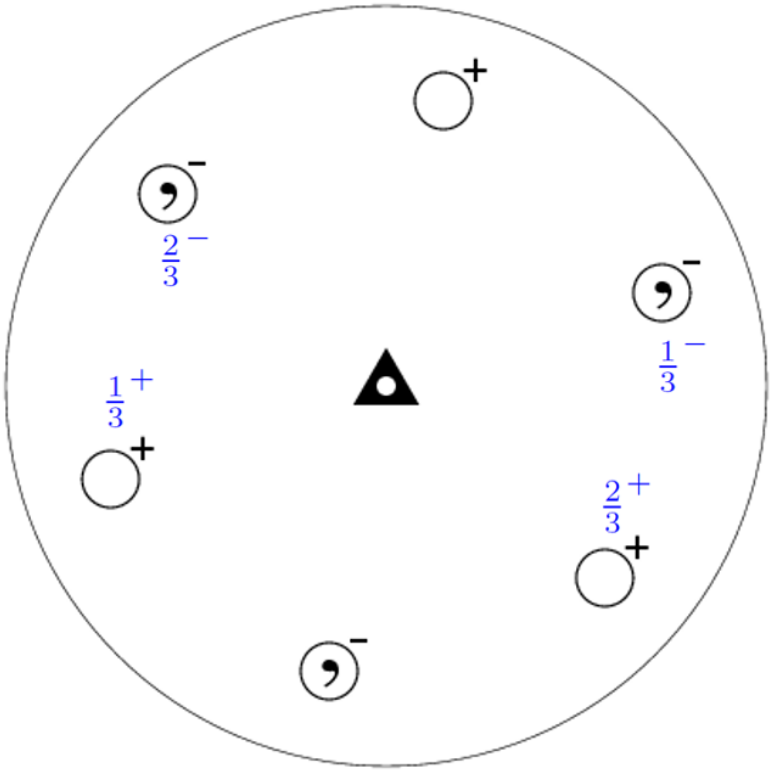

**17.3.53** **3** $\bar{3}$

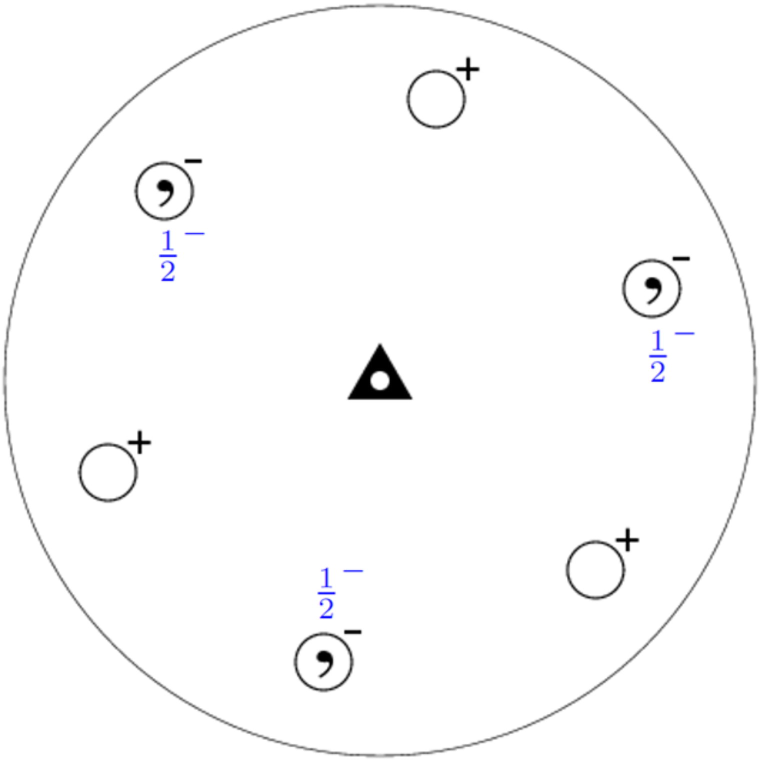

**17.4.54** **1** $\bar{3}$

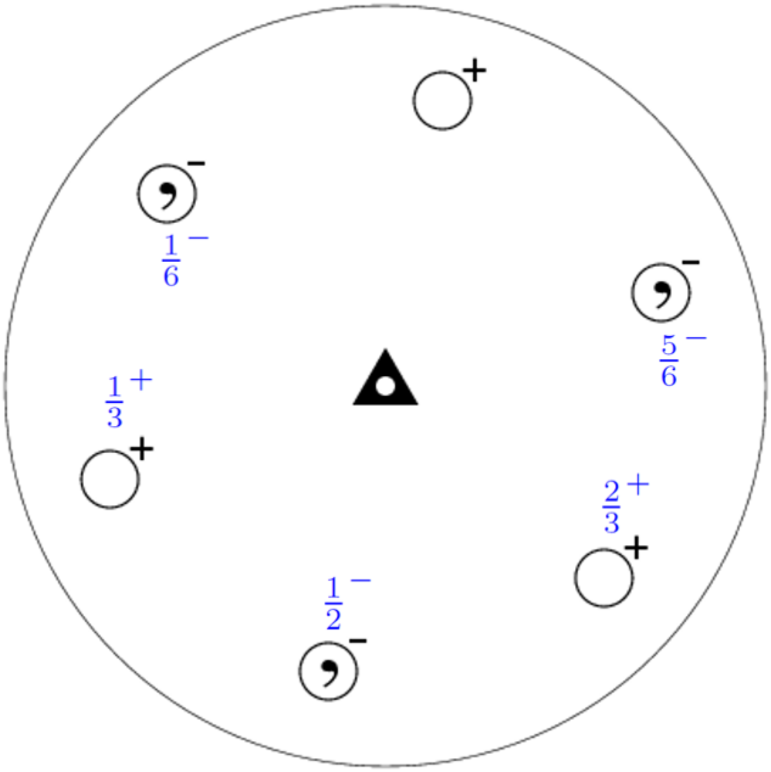

Supplement: Supplementary file 1 [file Stereographic_projections_1.pdf]
