# Supplementary material for: Spatio-temporal Symmetry - Point Groups with Time Translations
Source: arXiv:1701.04088 ancillary file (2017-09-21)

18.1.55

32

32

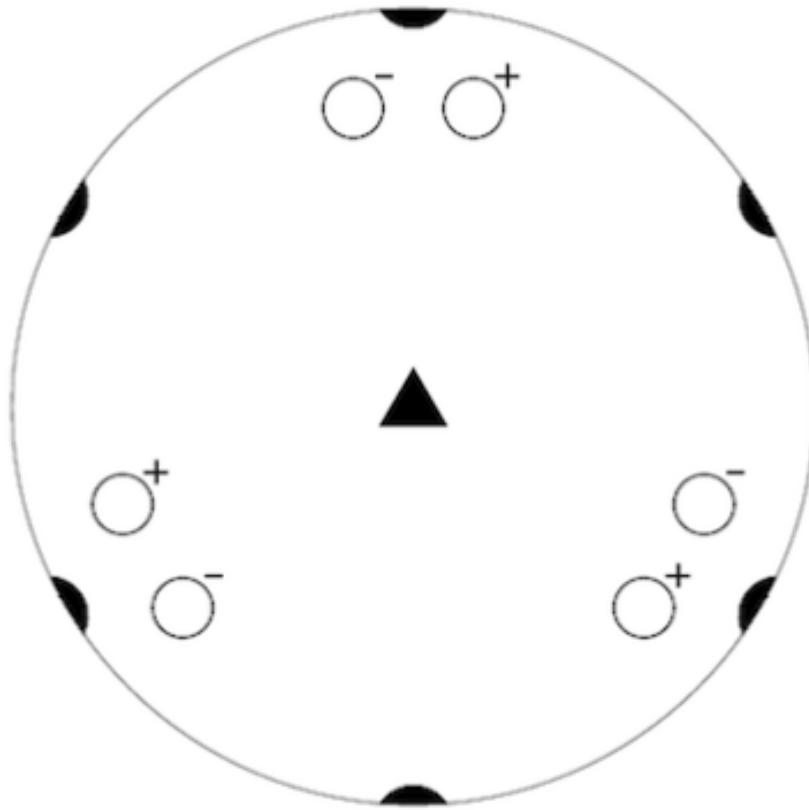

18.2.56

3

32

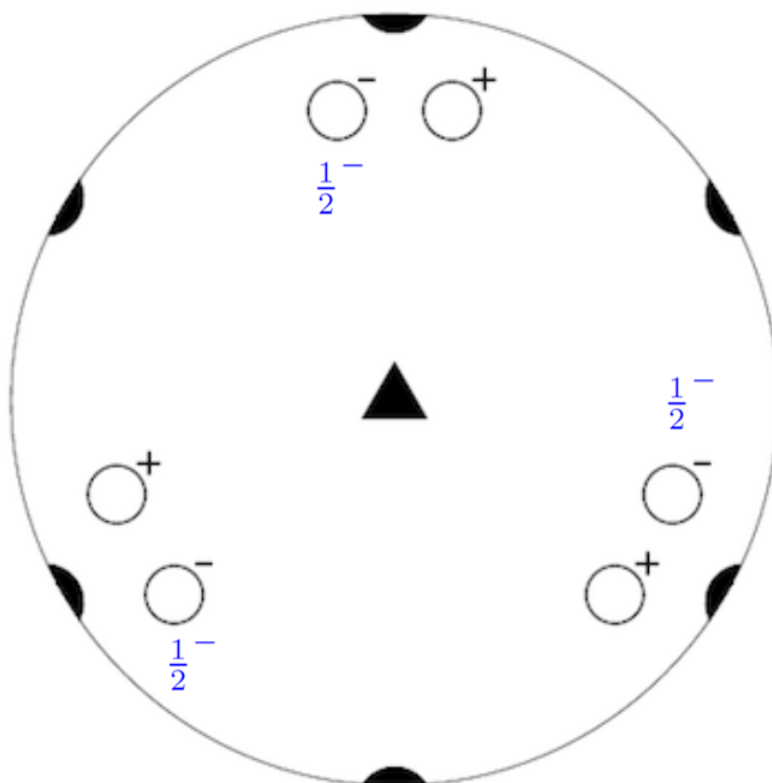

19.1.57

3m

3m

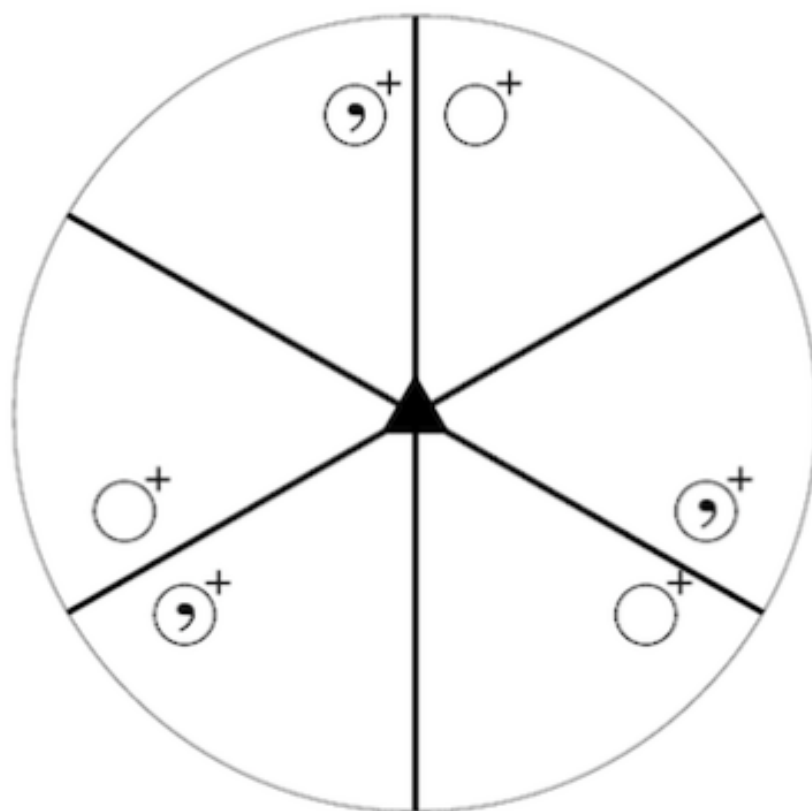

19.2.58

3

3m

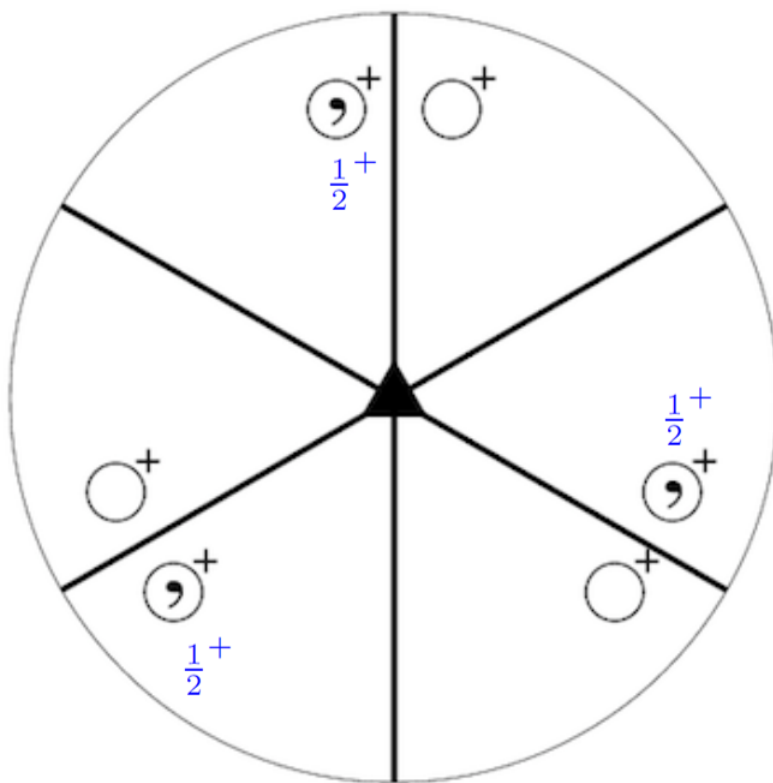

20.1.59

$\bar{3}m$

$\bar{3}m$

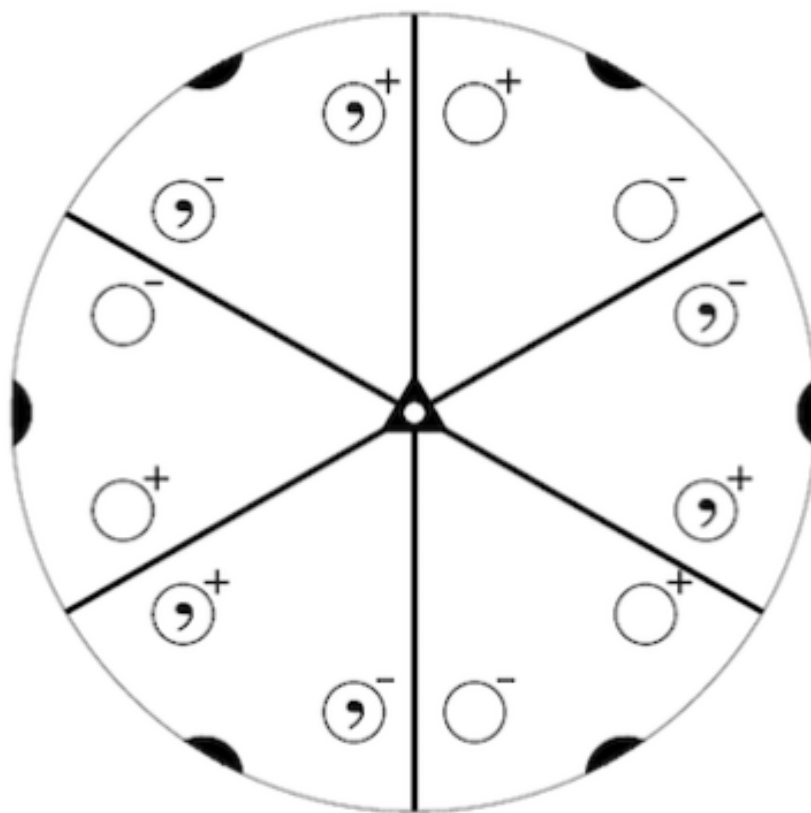

20.2.60

$\bar{3}$

$\bar{3}m$

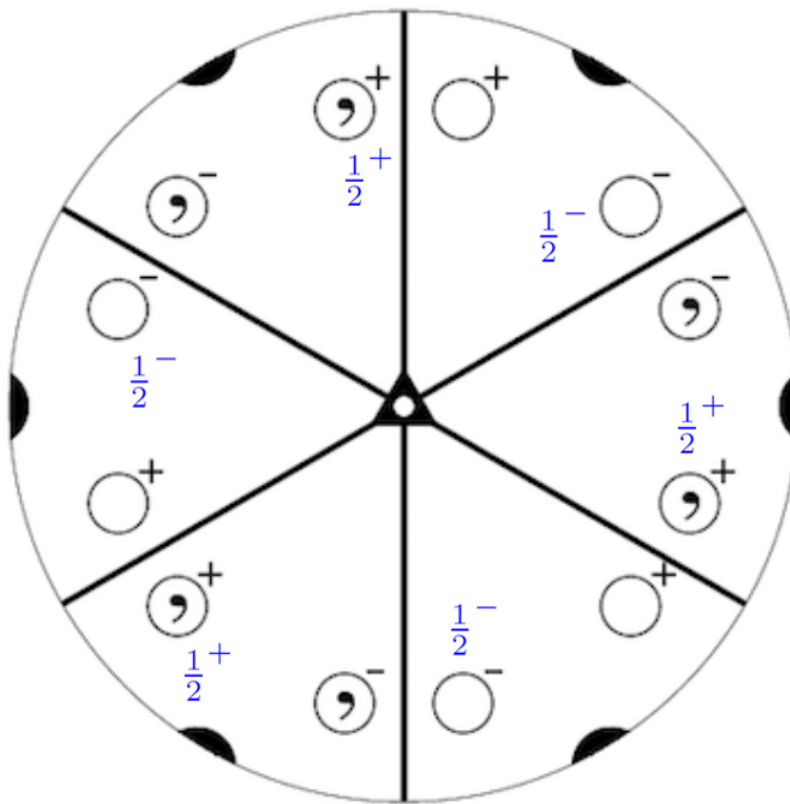

20.3.61

32

$\bar{3}m$

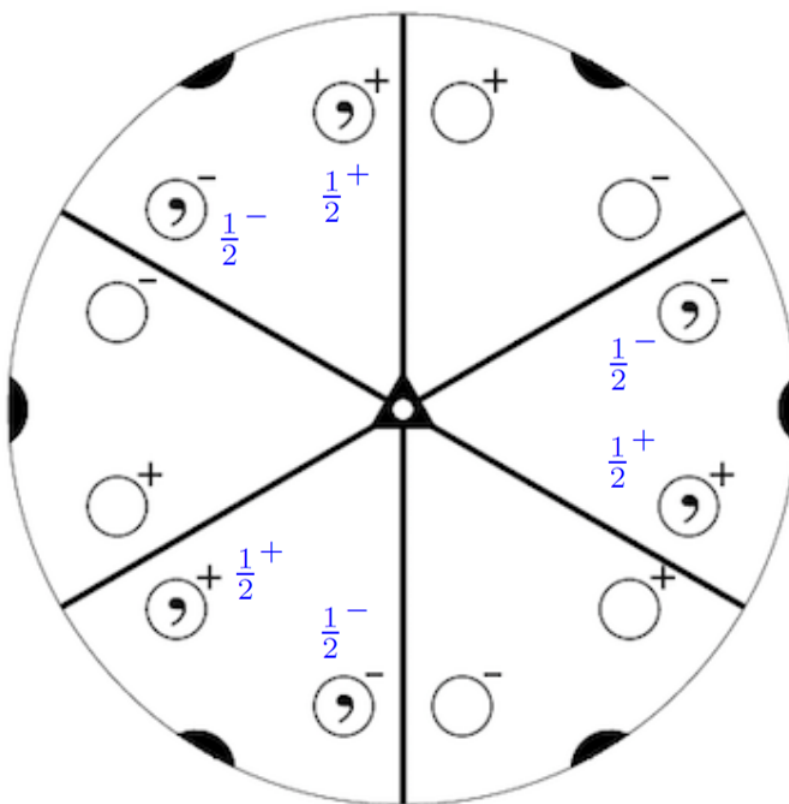

20.4.62

3m

$\bar{3}m$

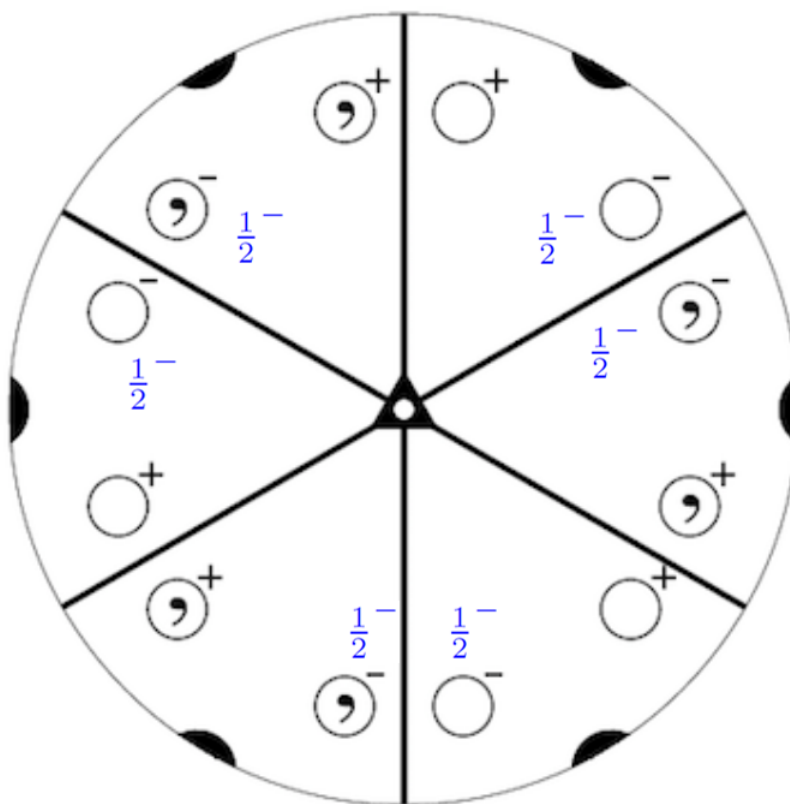



21.1.63

6

6

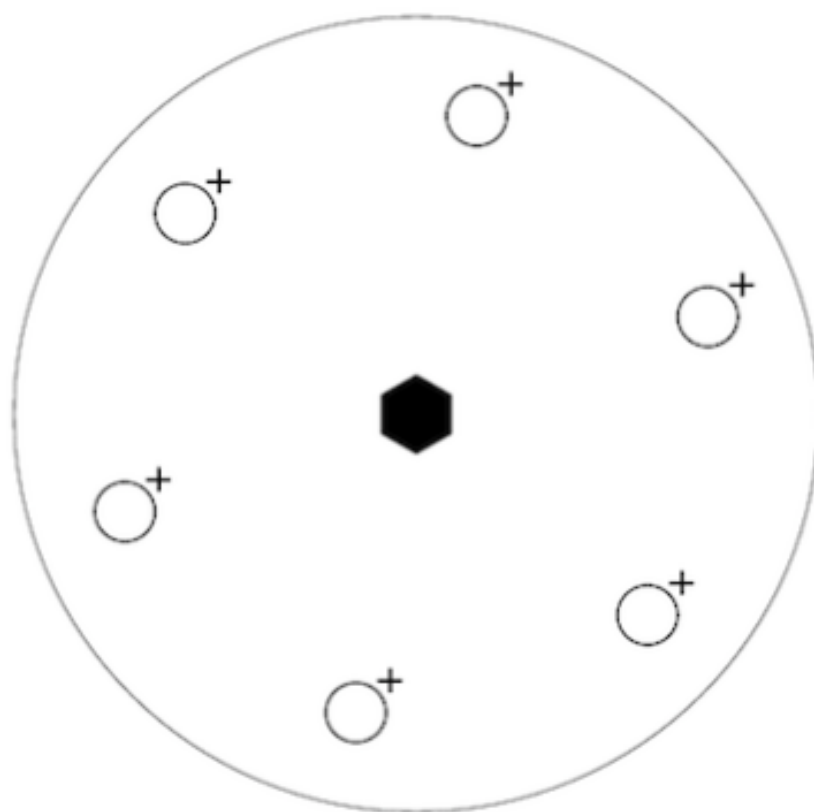

21.2.64

3

6

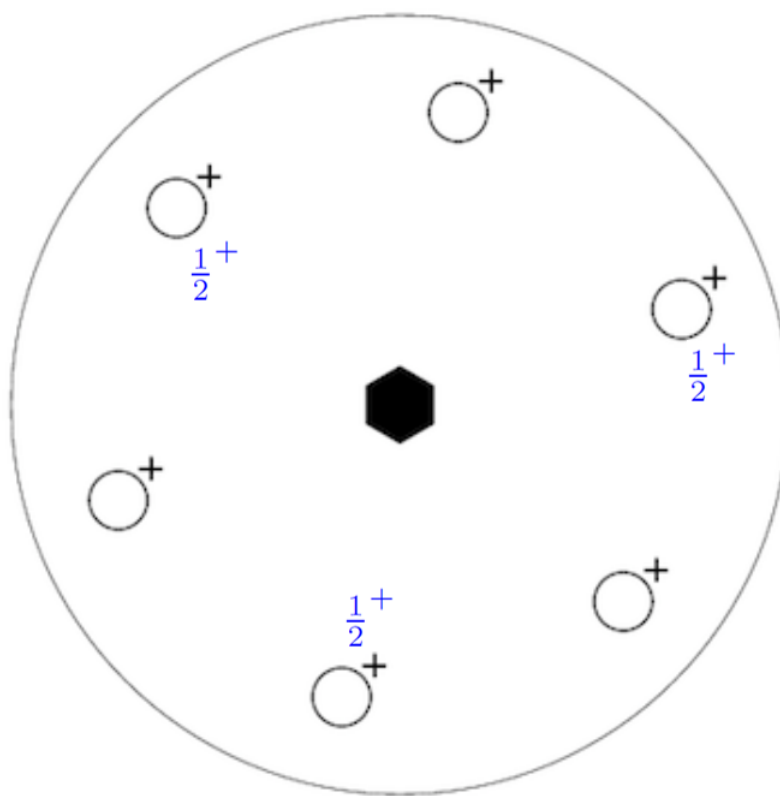

21.3.65

1

6

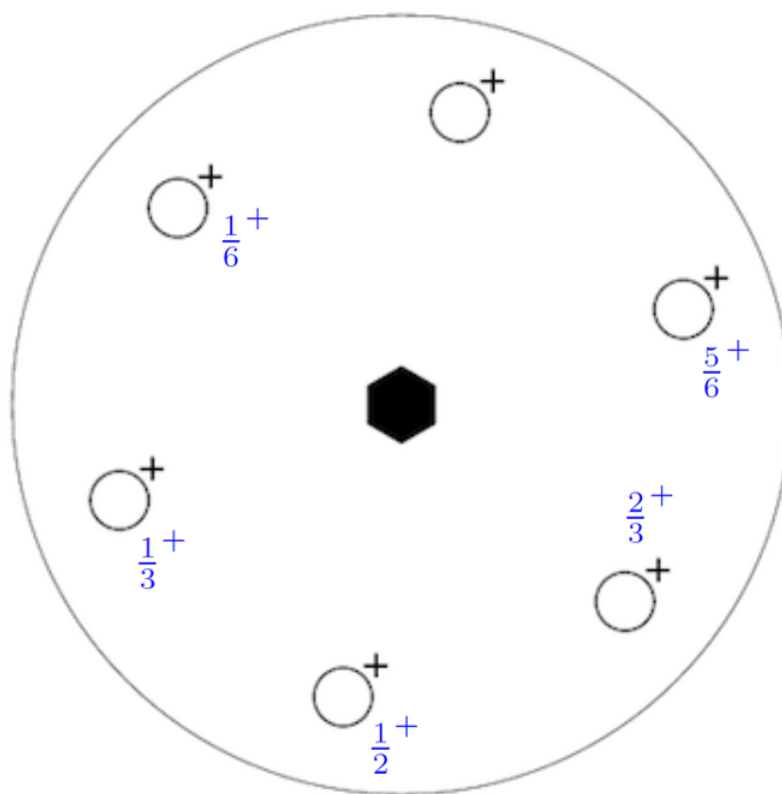

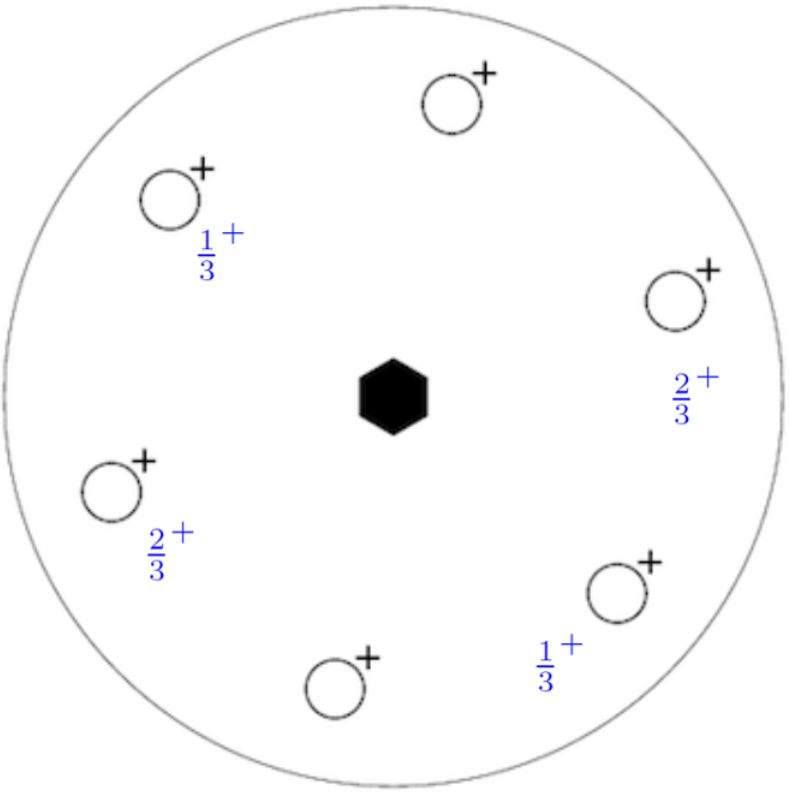

22.1.67

$\bar{6}$

$\bar{6}$

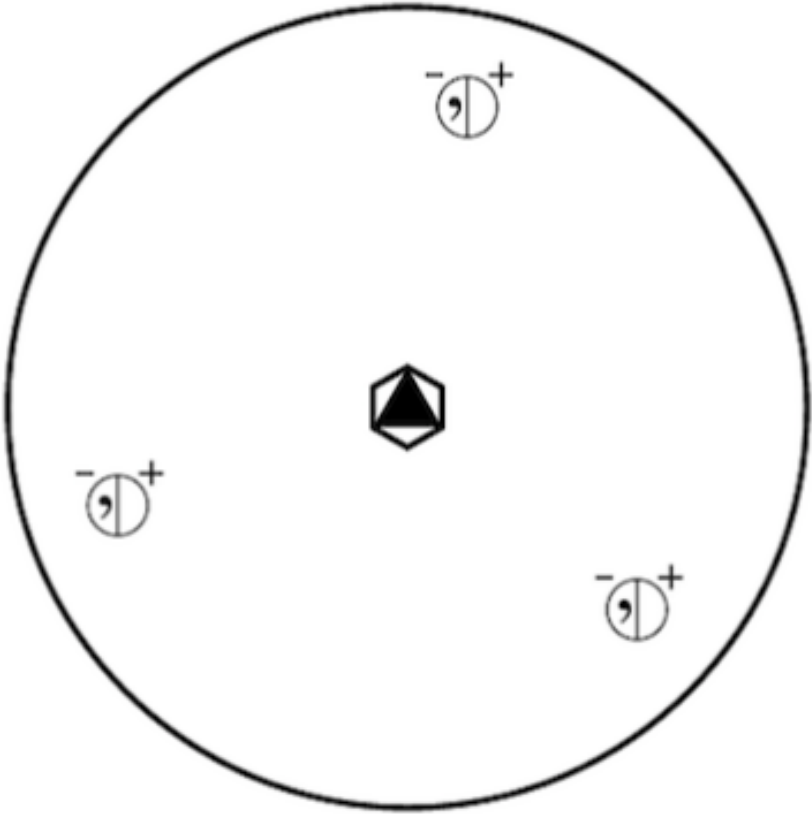

22.2.68

m

$\bar{6}$

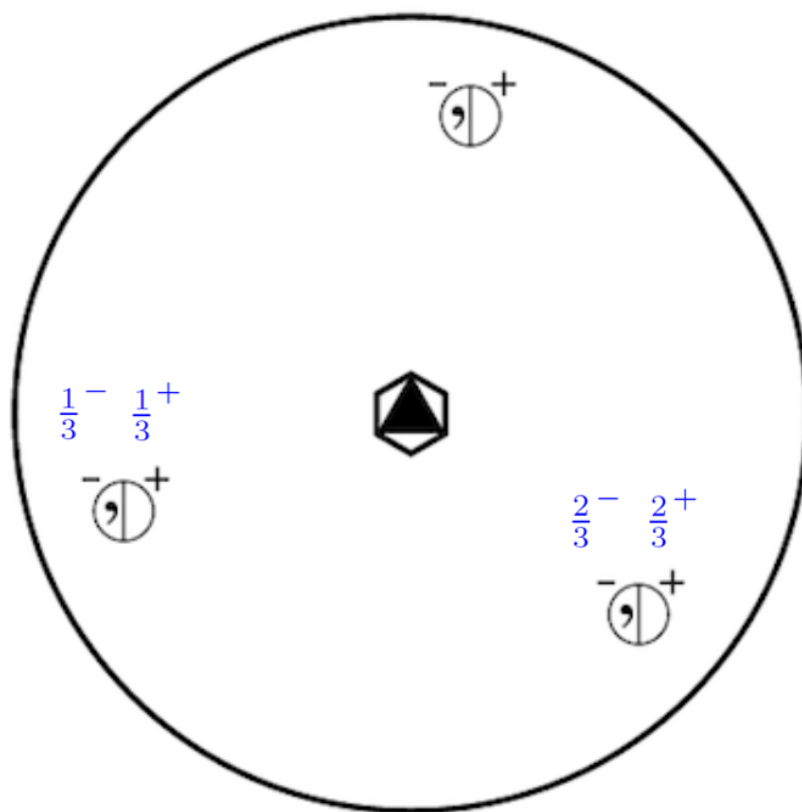

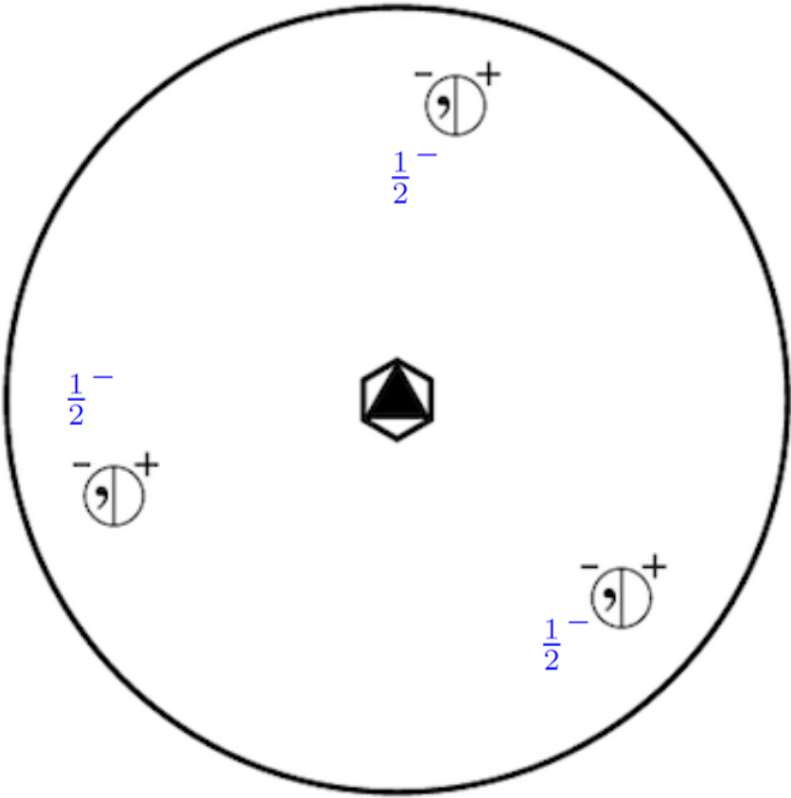

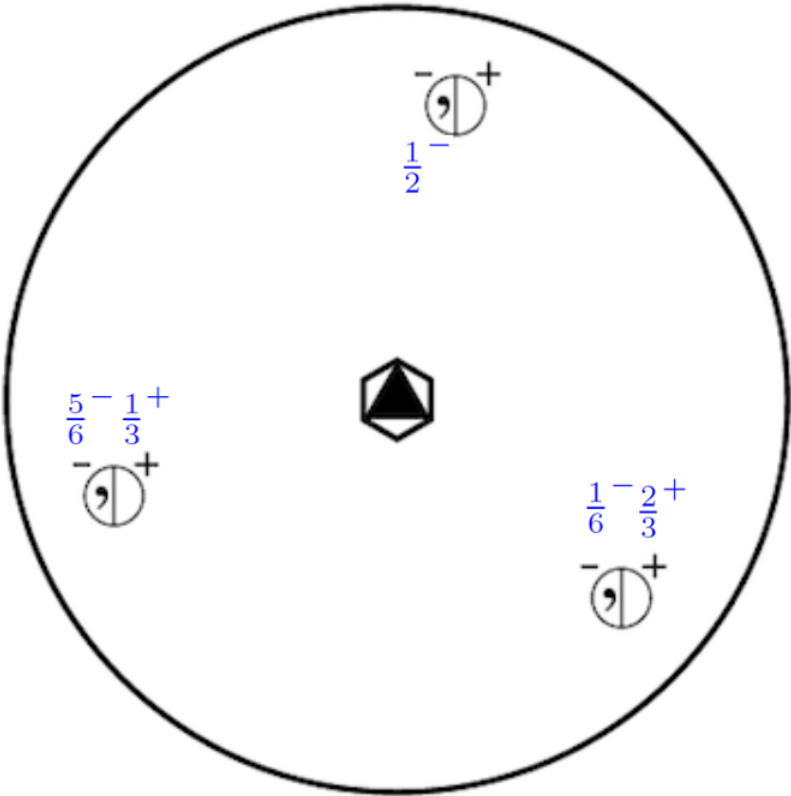



23.1.71

6/m

6/m

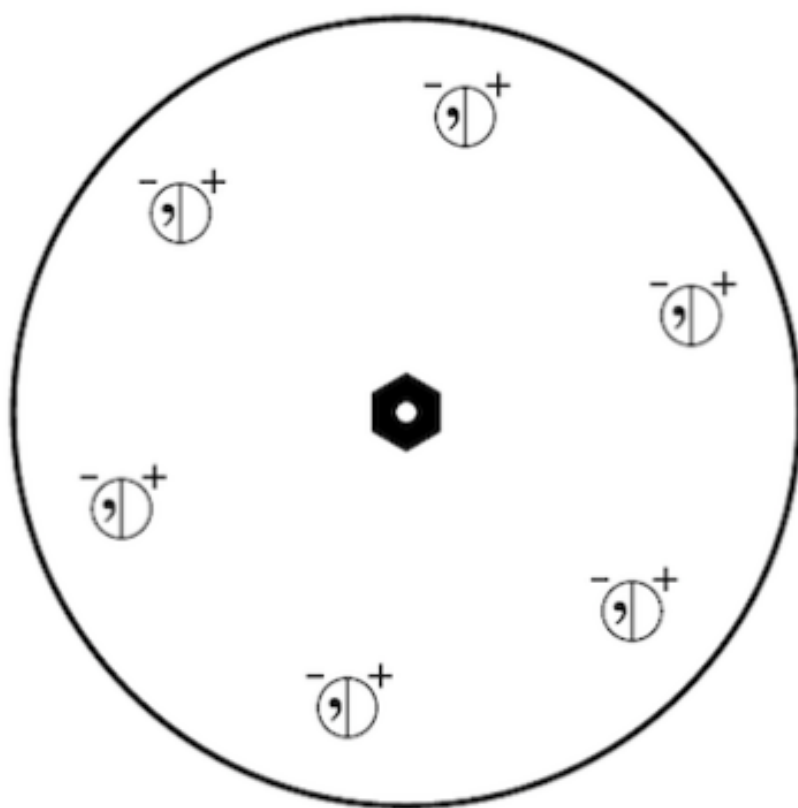

23.2.72

$\bar{3}$

6/m

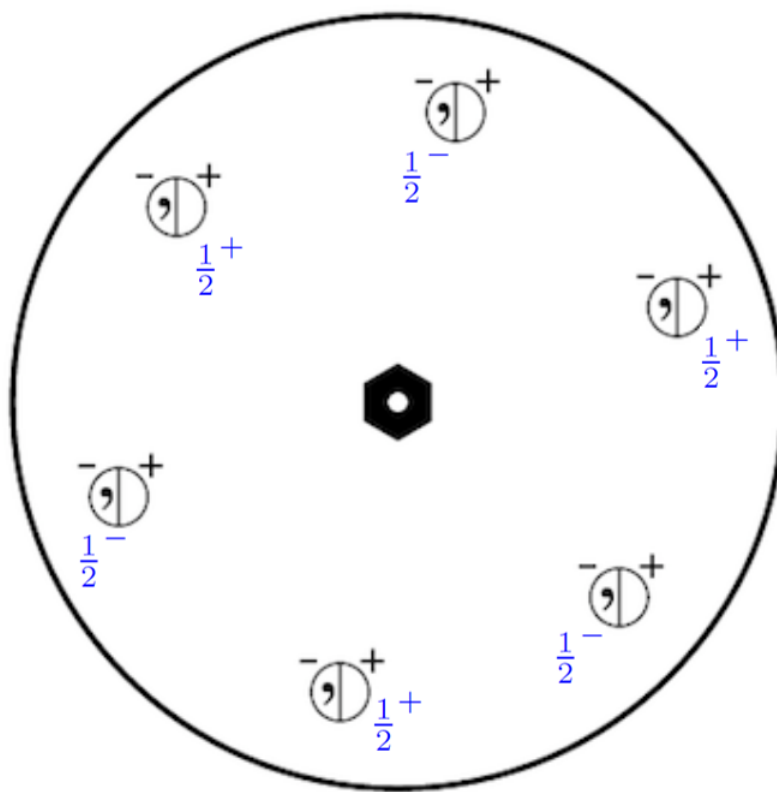

23.3.73

$\bar{1}$

6/m

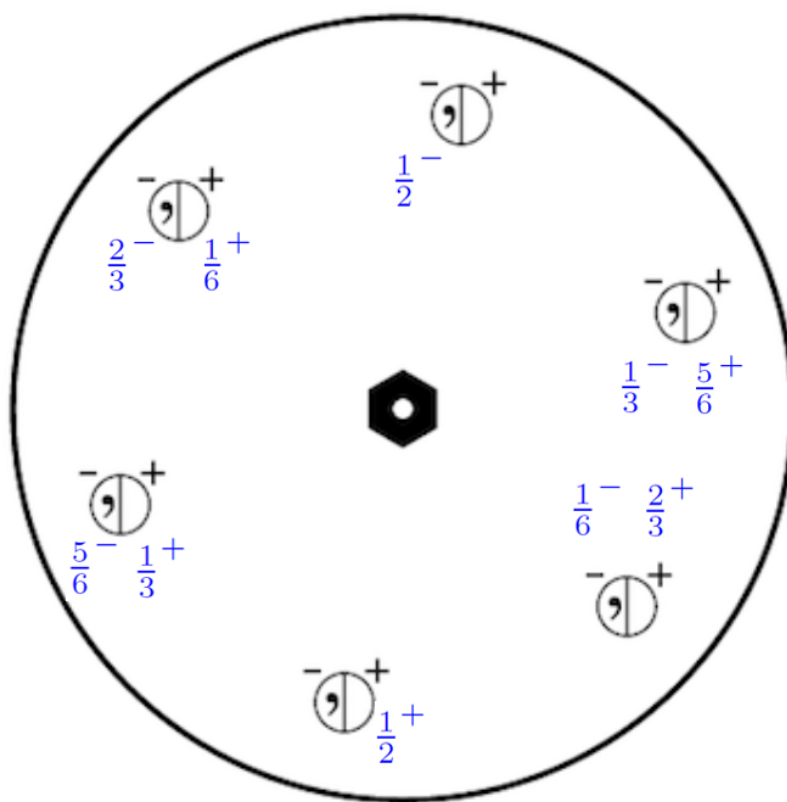

23.4.74

2/m

6/m

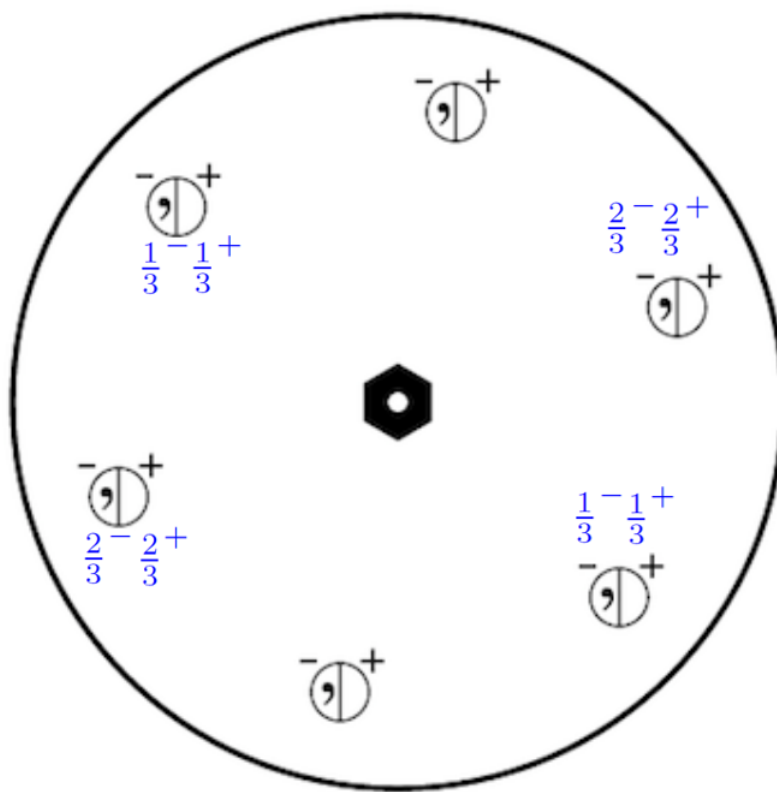

23.5.75

6

6/m

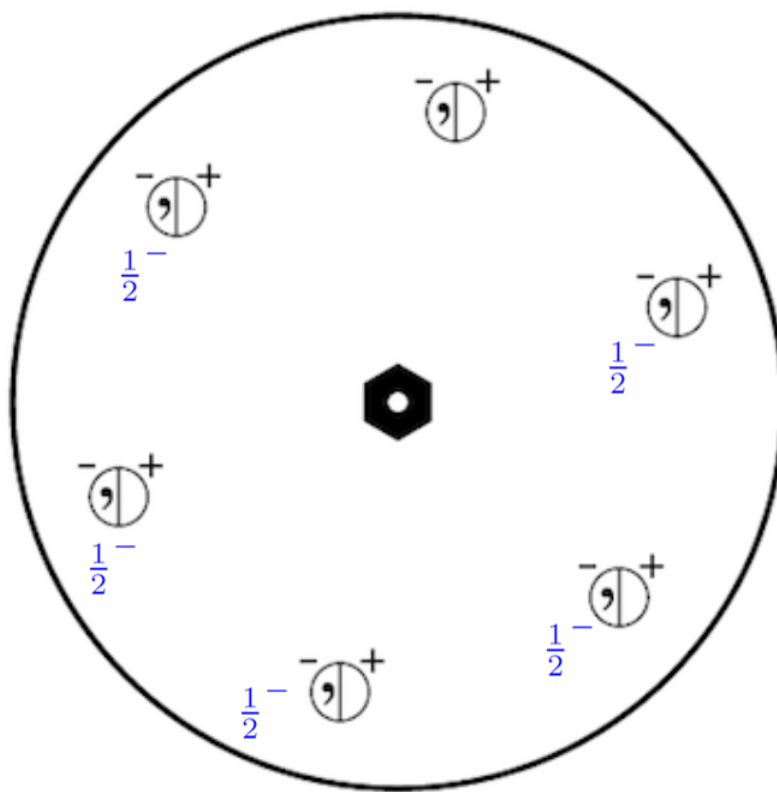

23.6.76

$\bar{6}$

6/m

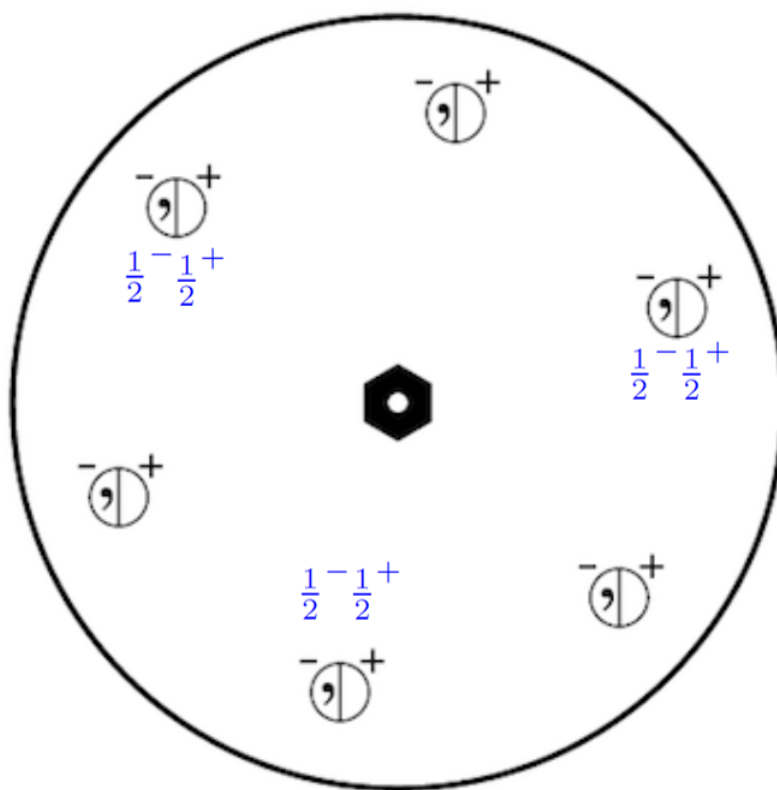

23.7.77

m

6/m

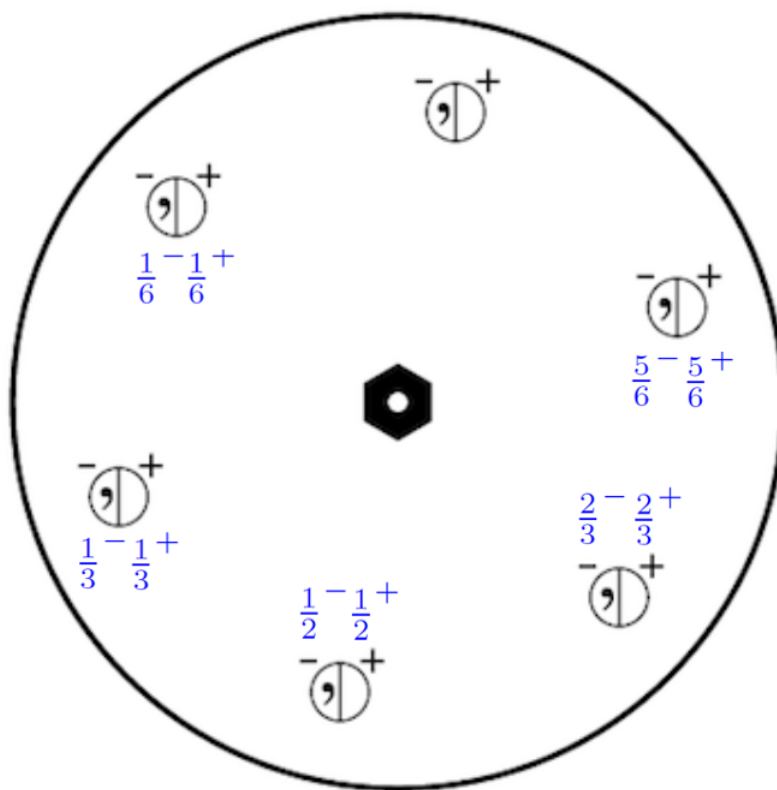

23.8.78

2

6/m

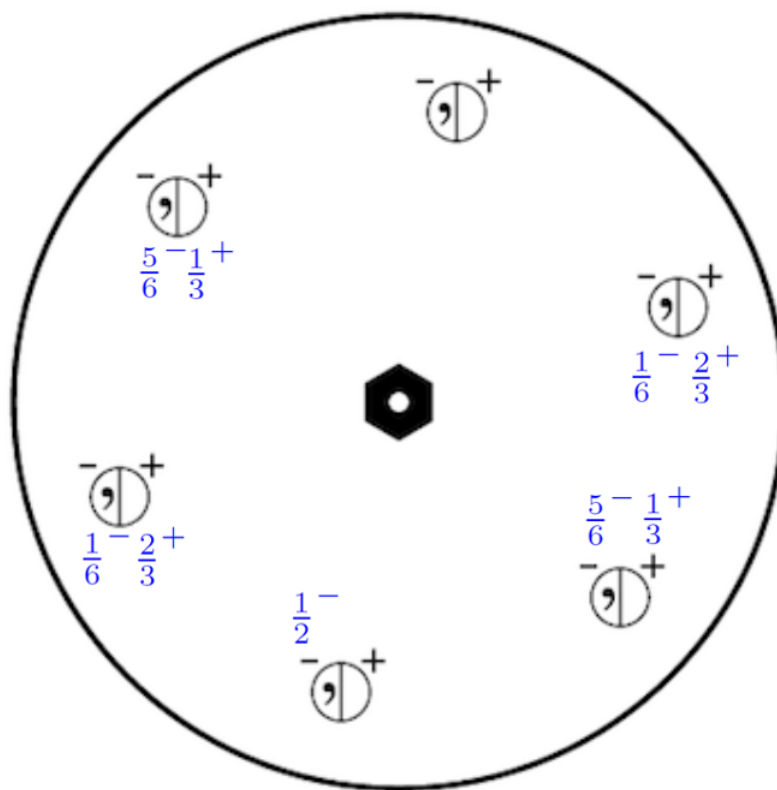



24.1.79

622

622

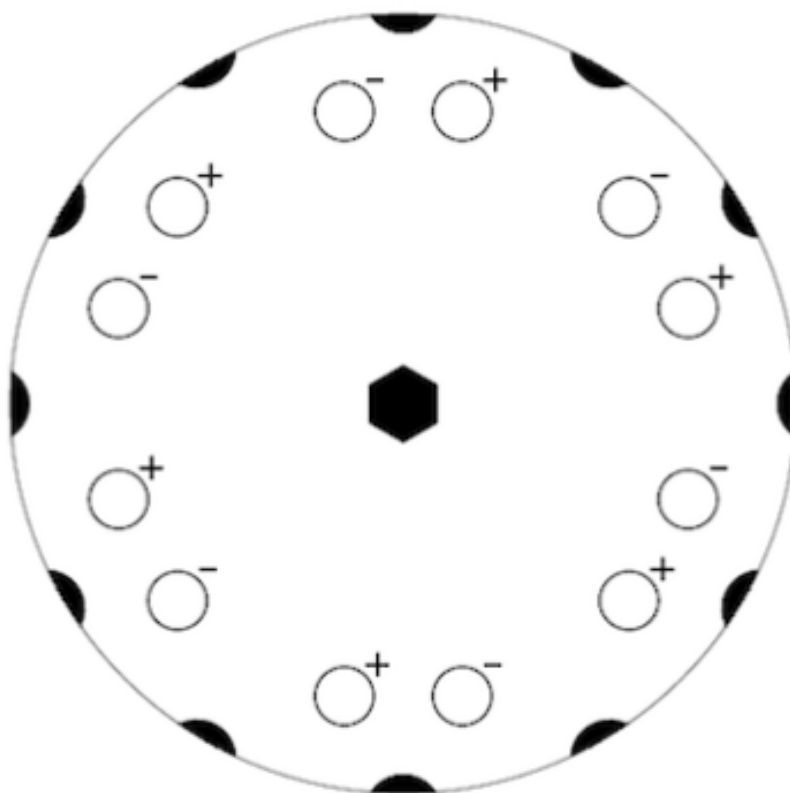

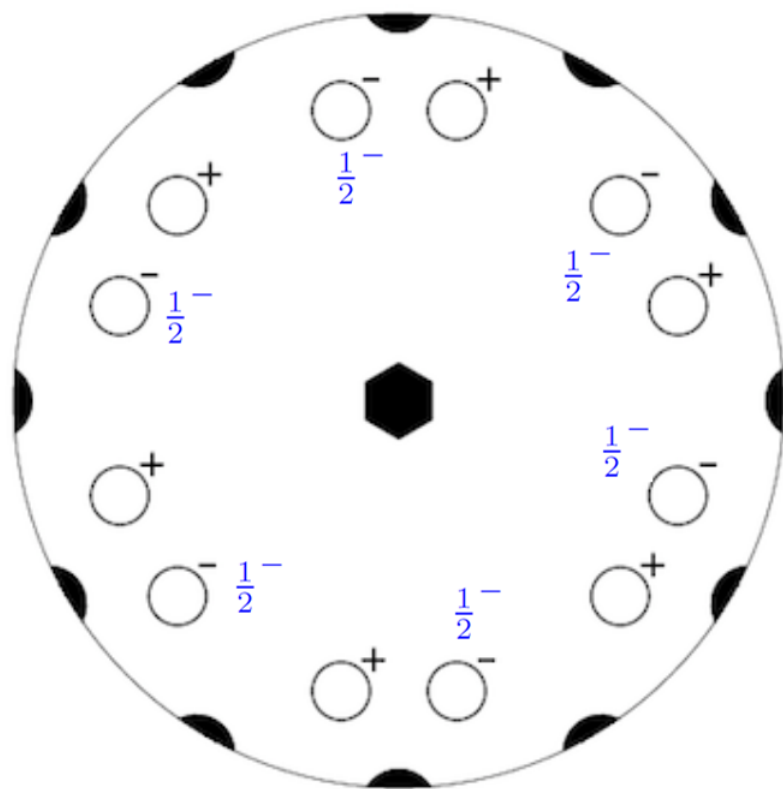



25.1.82

6mm

6mm

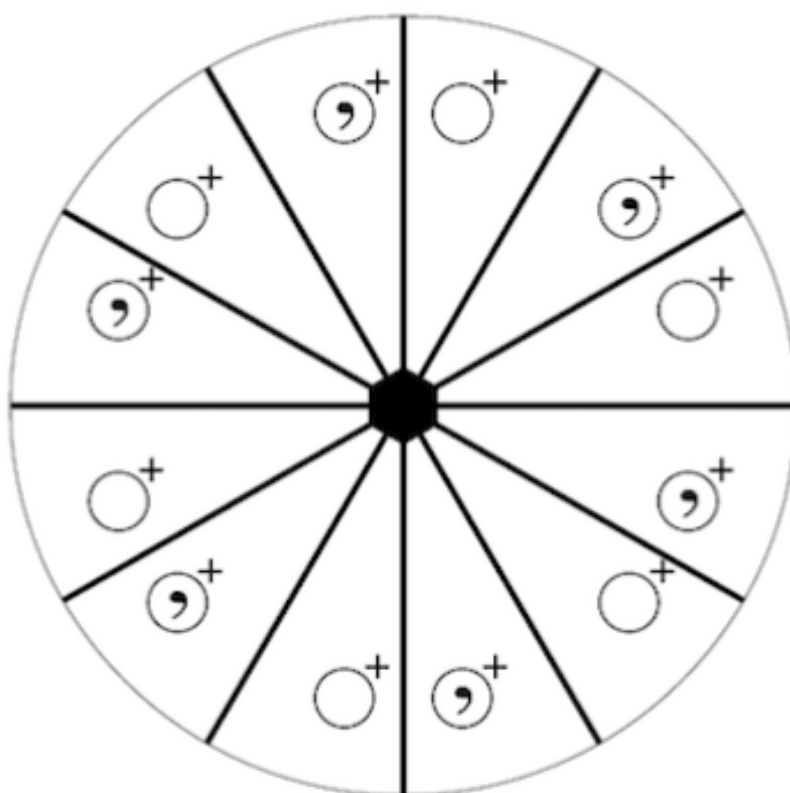

25.2.83

6

6mm

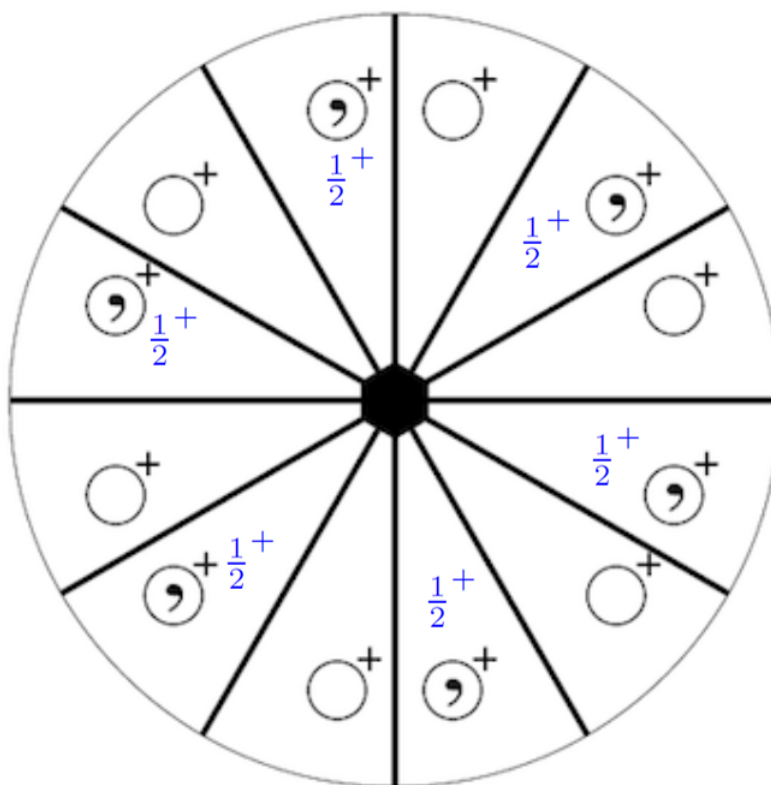

25.3.84

3m

6mm

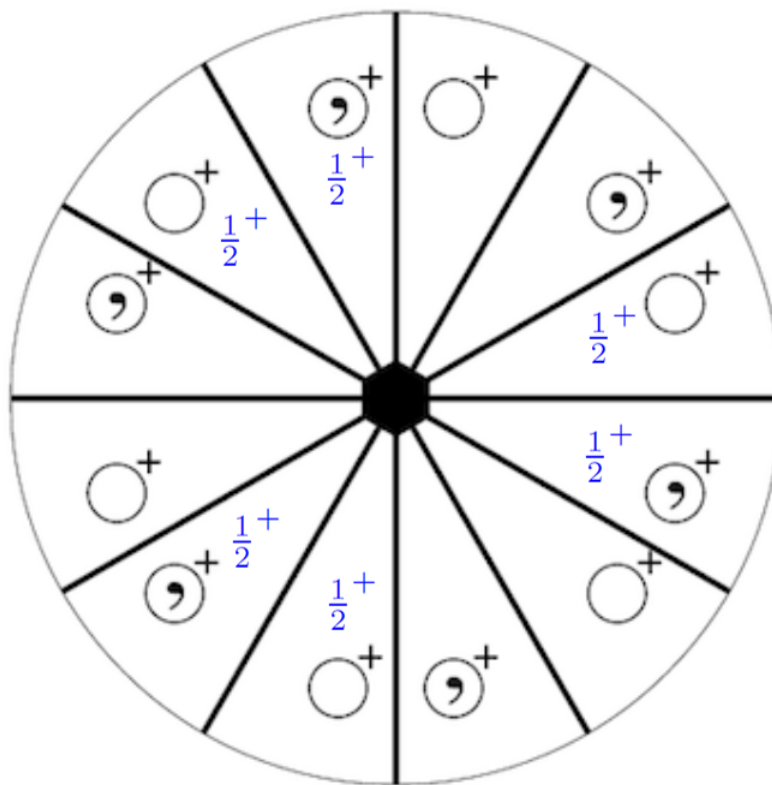

26.1.85

$\bar{6}2m$

$\bar{6}2m$

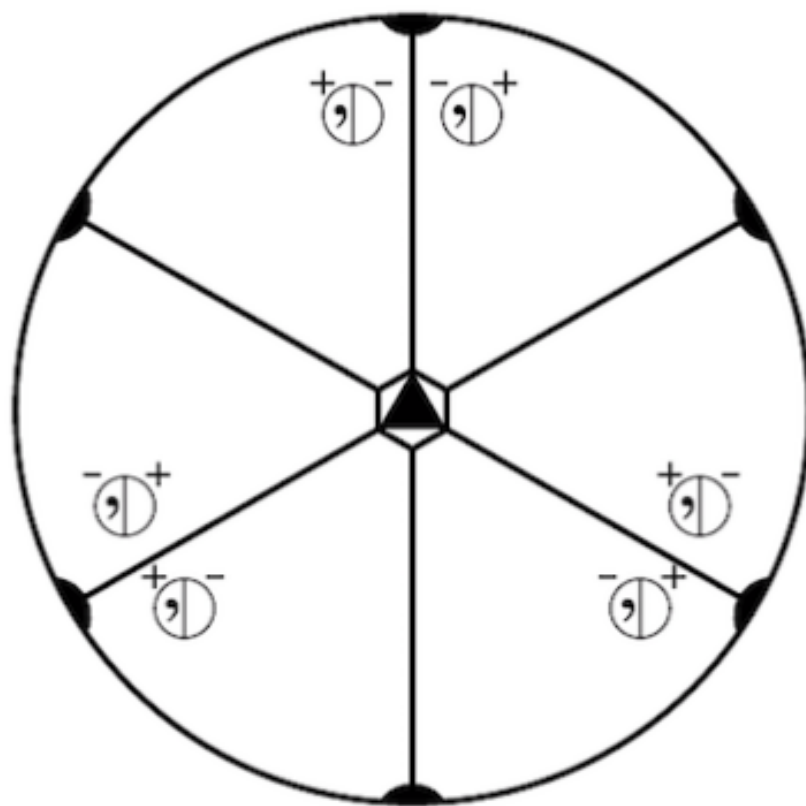

26.2.86

$\bar{6}$

$\bar{6}2m$

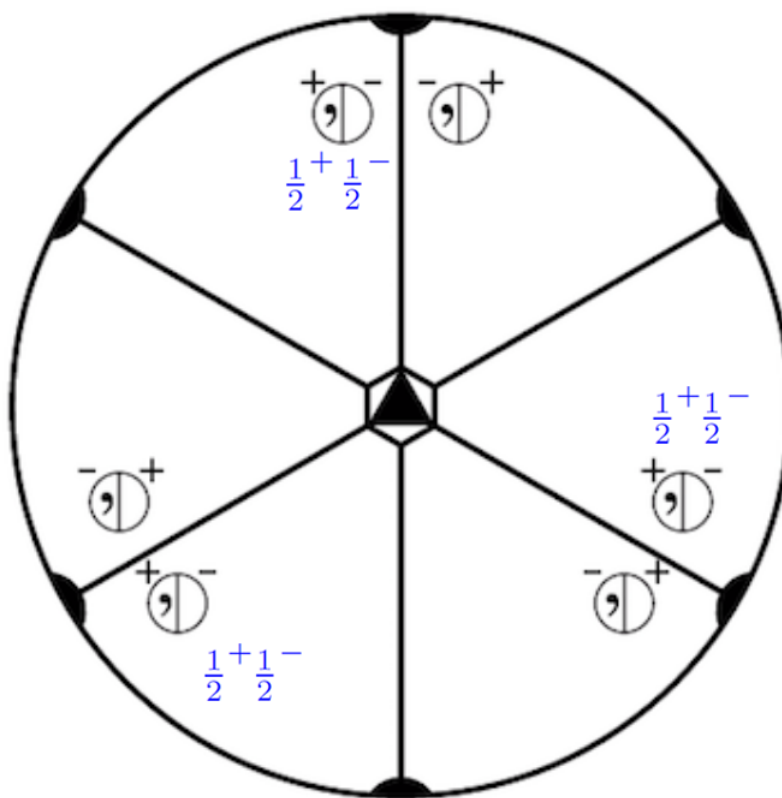



26.3.87

32

$\bar{6}2m$

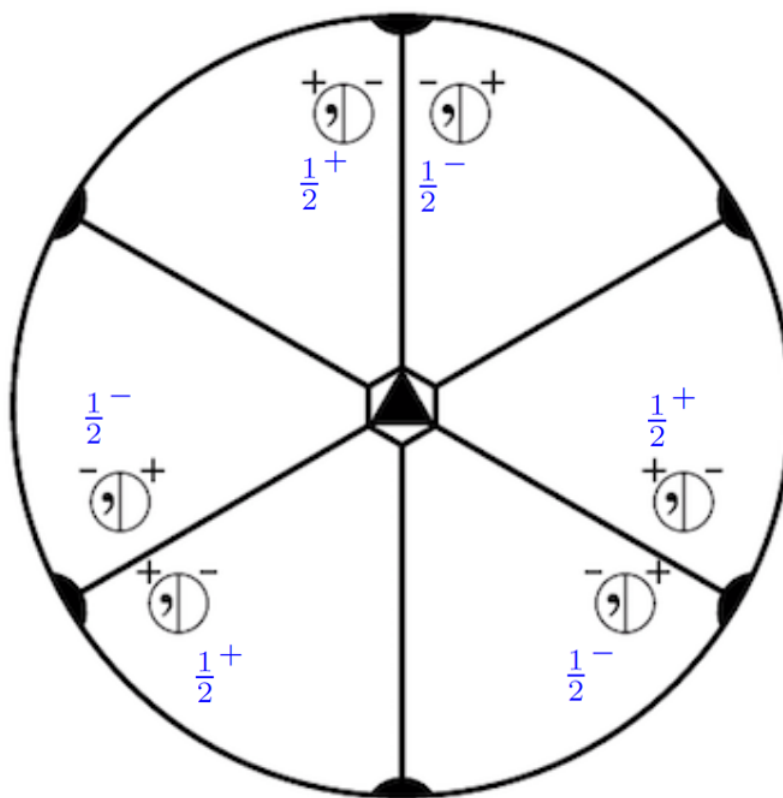

26.4.88

3m

$\bar{6}2m$

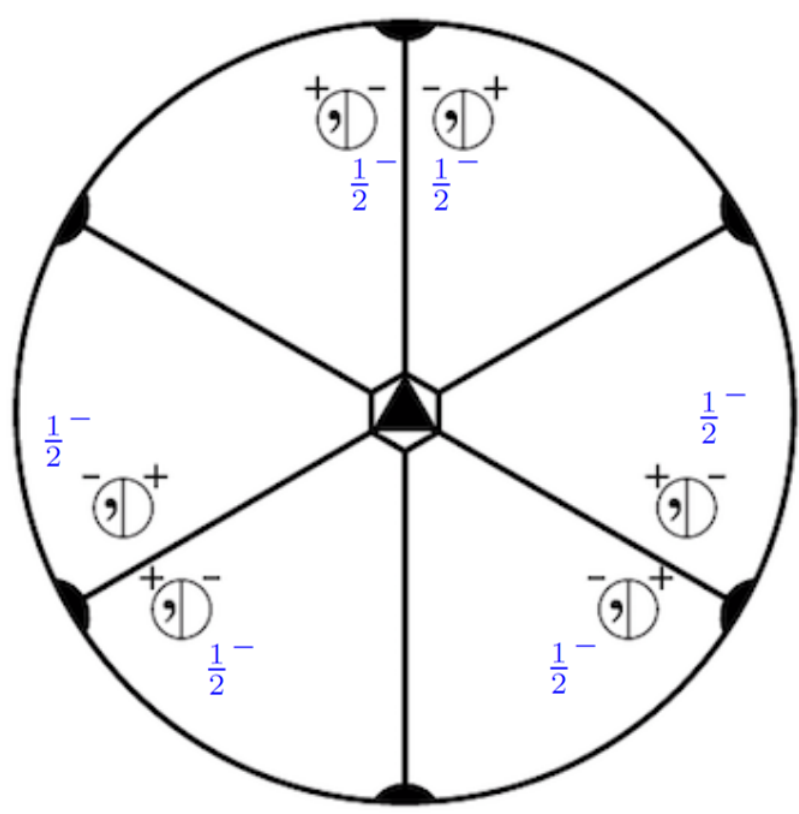

27.1.89

6/mmm

6/mmm

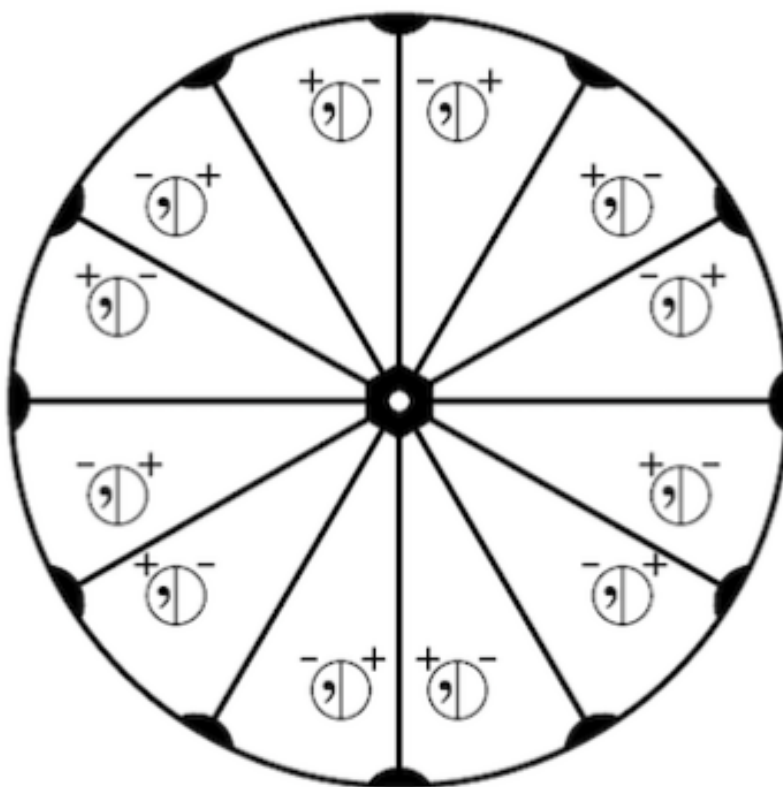

27.2.90

6

6/mmm

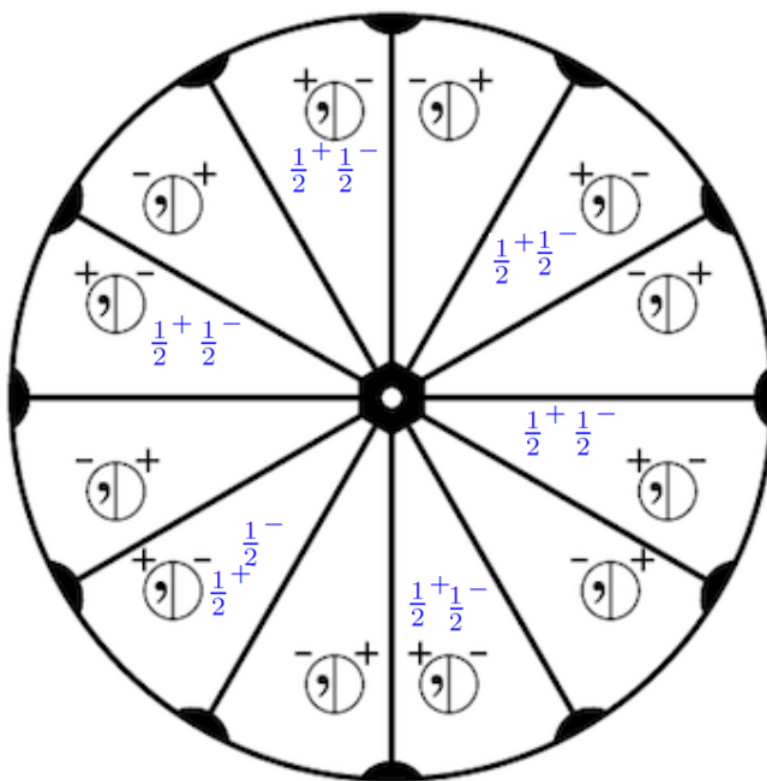

27.3.91

32

6/mmm

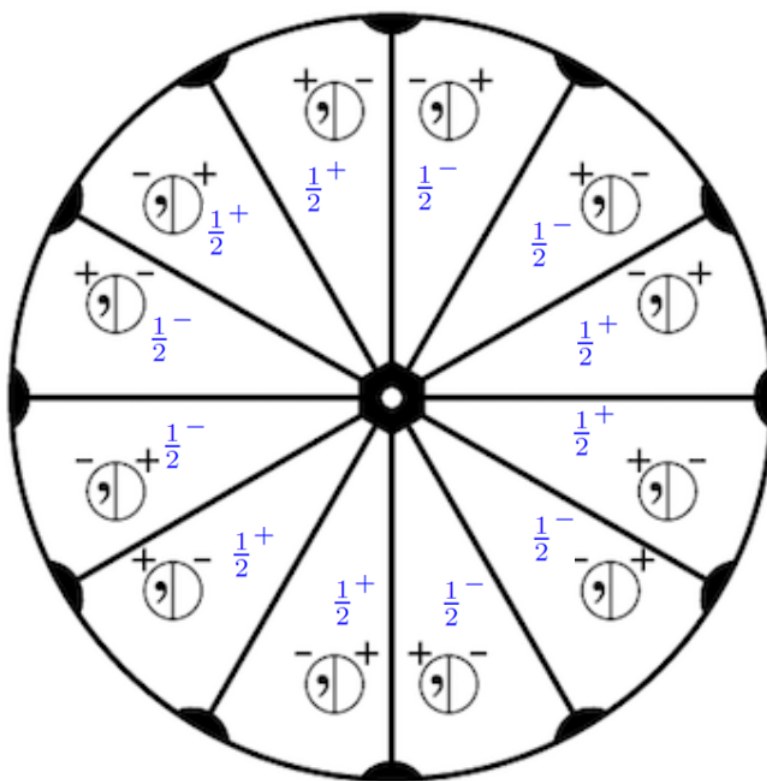

27.4.92

622

6/mmm

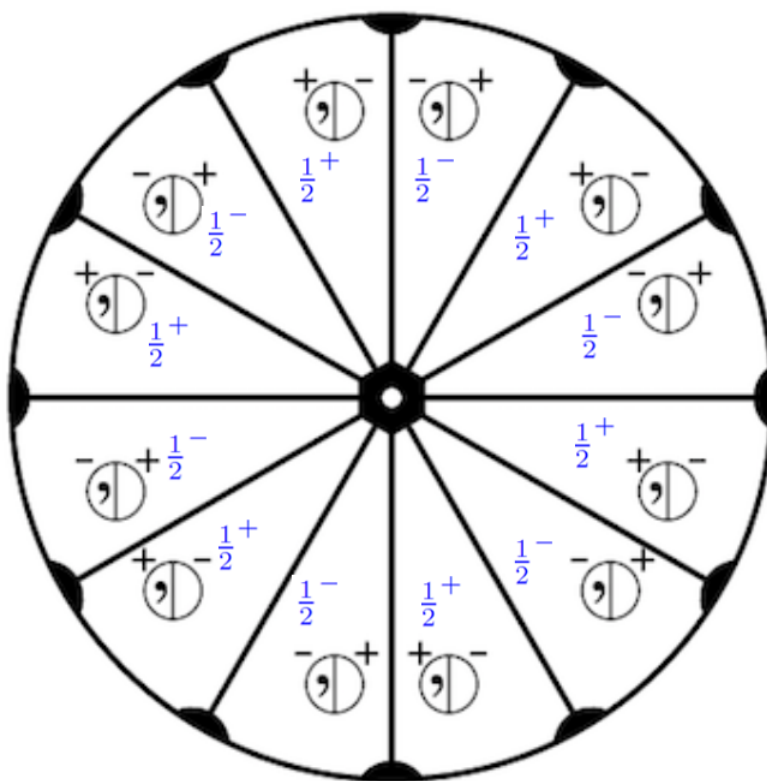

27.5.93

6mm

6/mmm

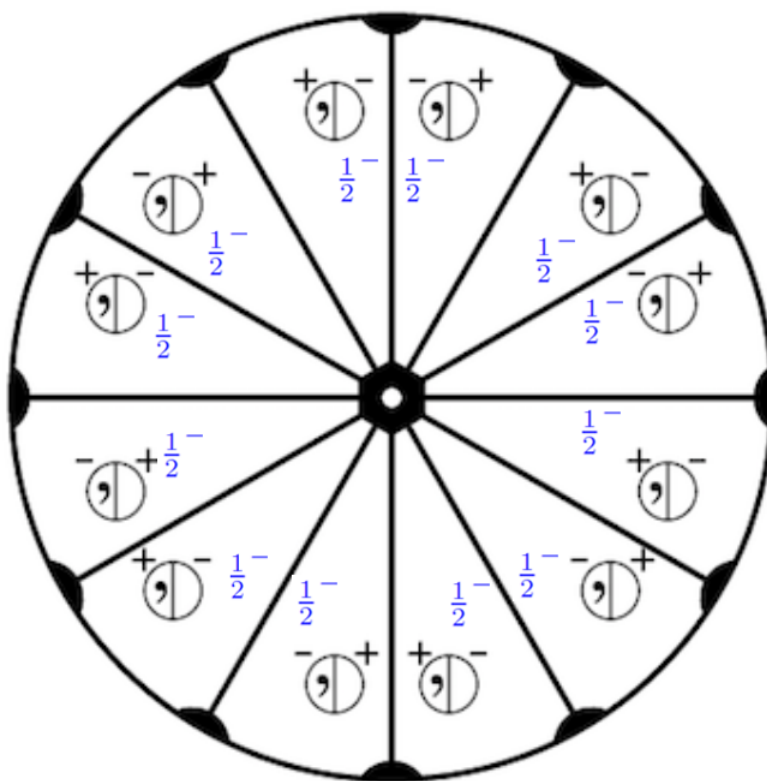

27.6.94

$\bar{6}2m$

$6/mmm$

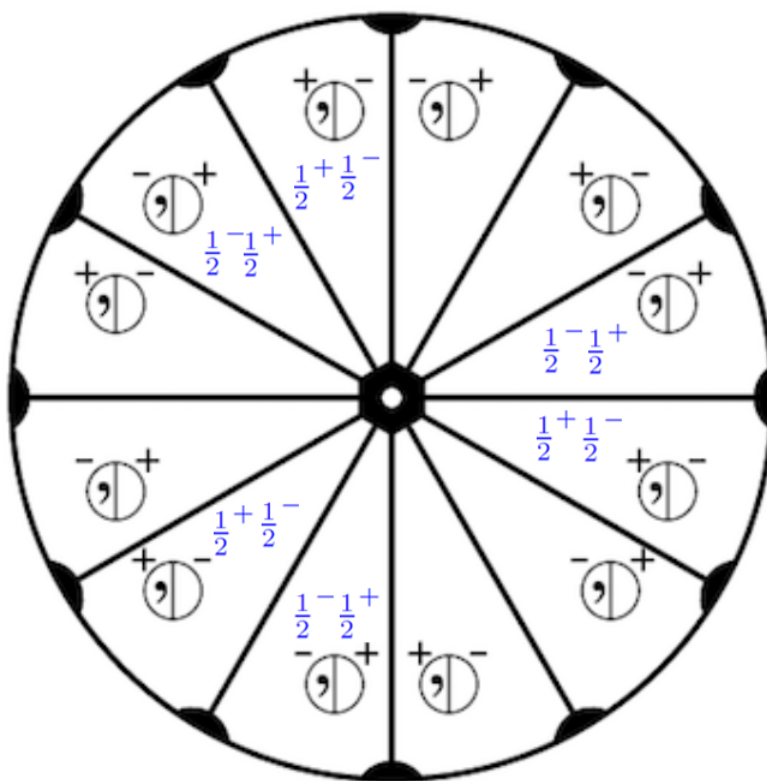



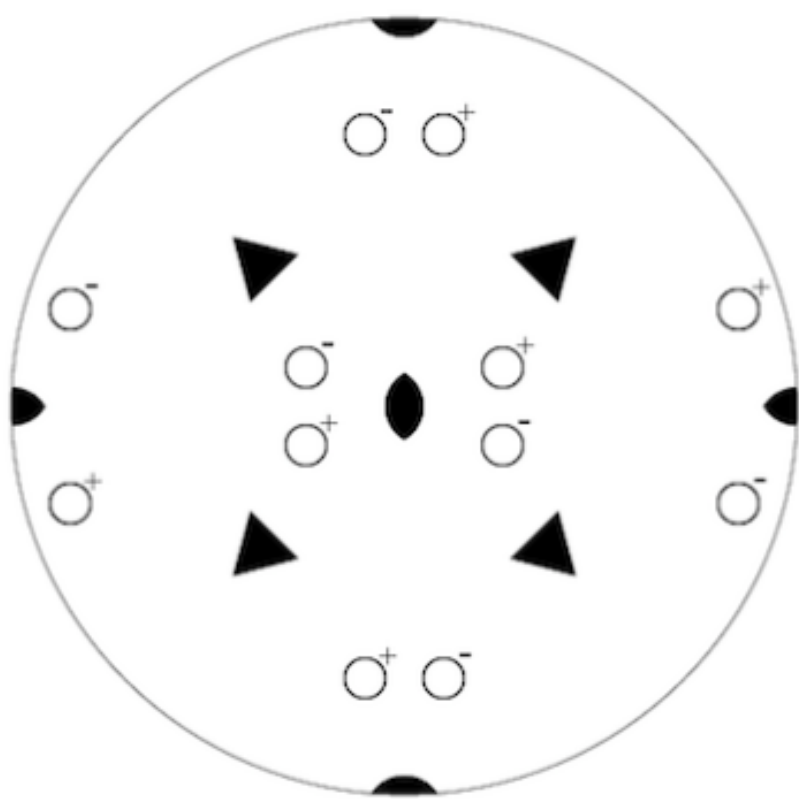

28.2.96

222

23

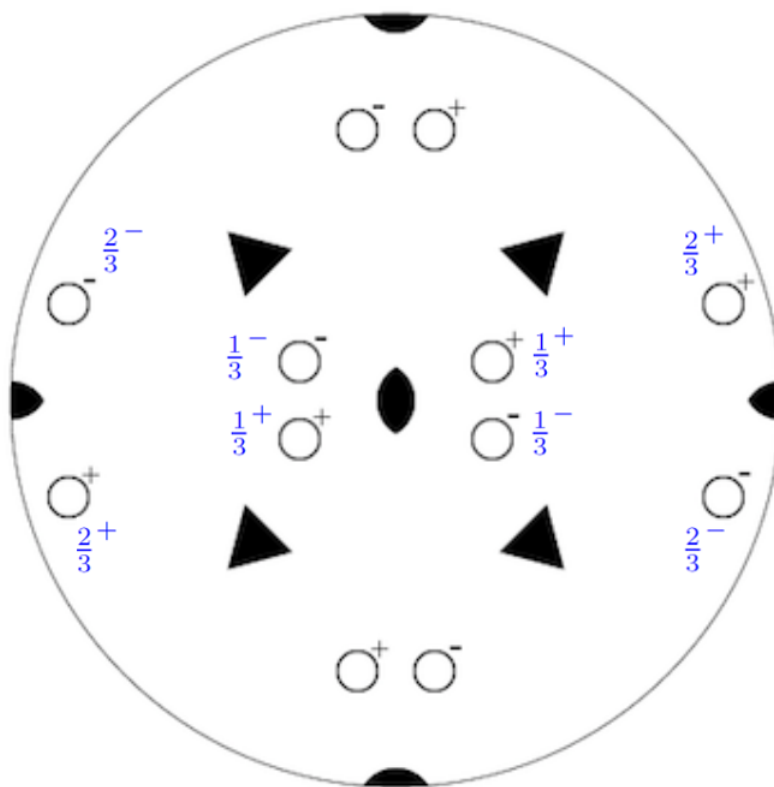

29.1.97

$m\bar{3}$

$m\bar{3}$

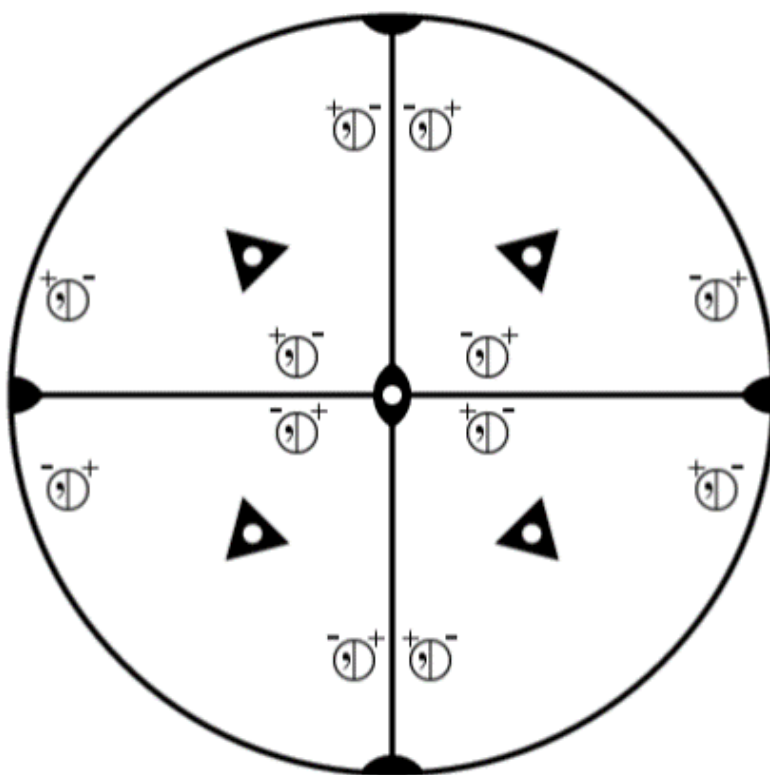

29.2.98

mmm

$m\bar{3}$

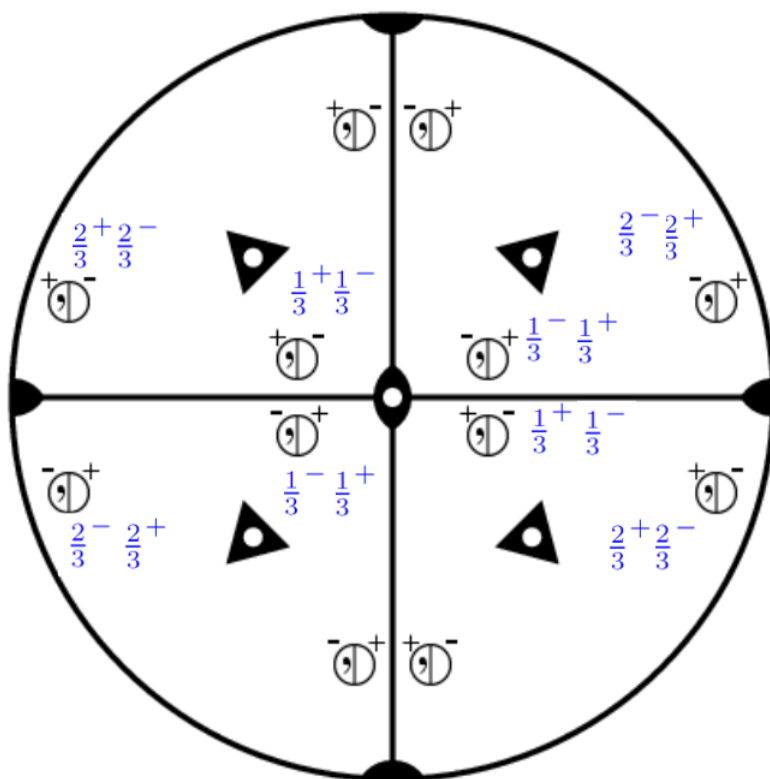

29.3.99

23

$m\bar{3}$

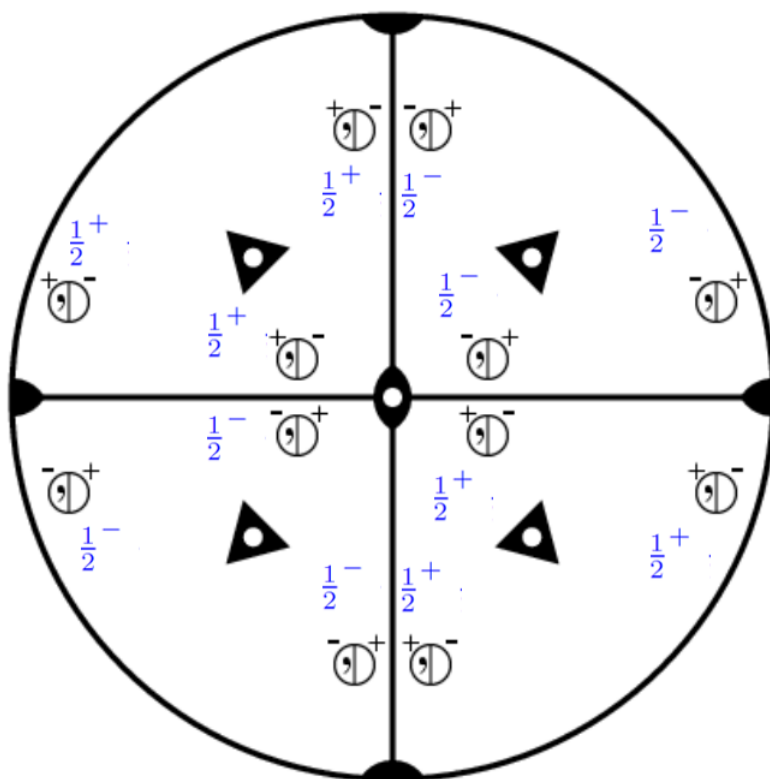

29.4.100

222

$m\bar{3}$

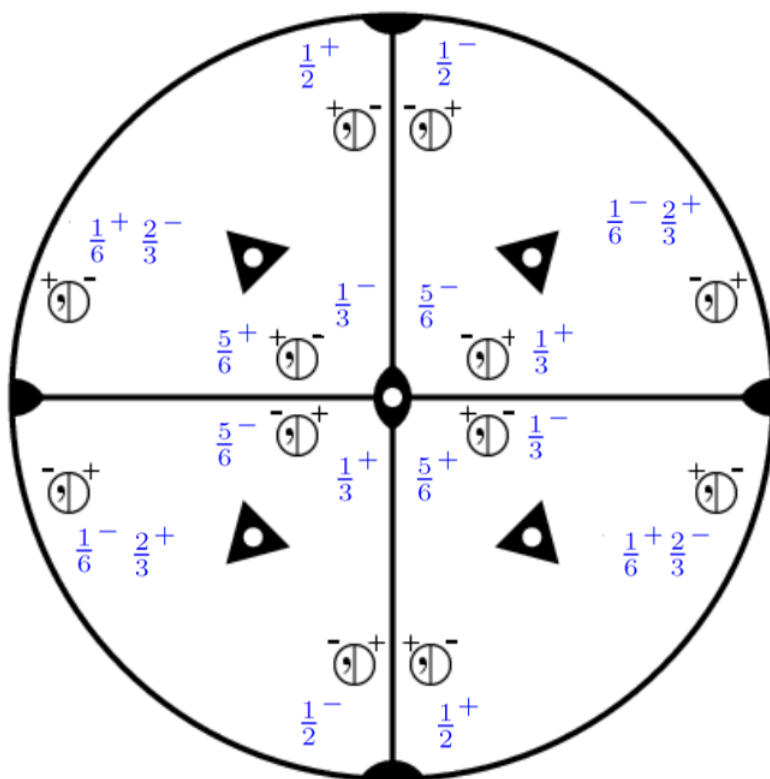

30.1.101

432

432

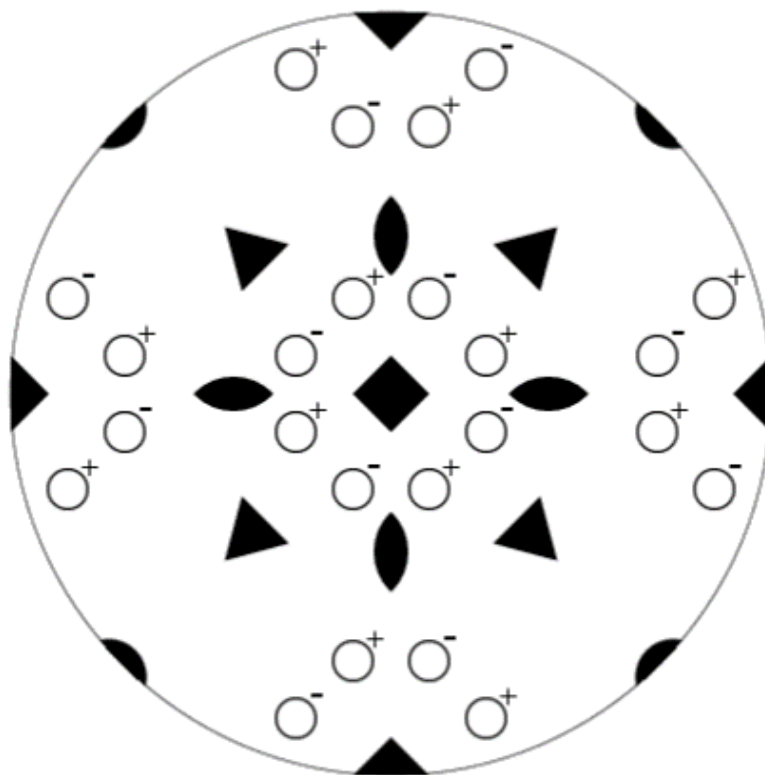

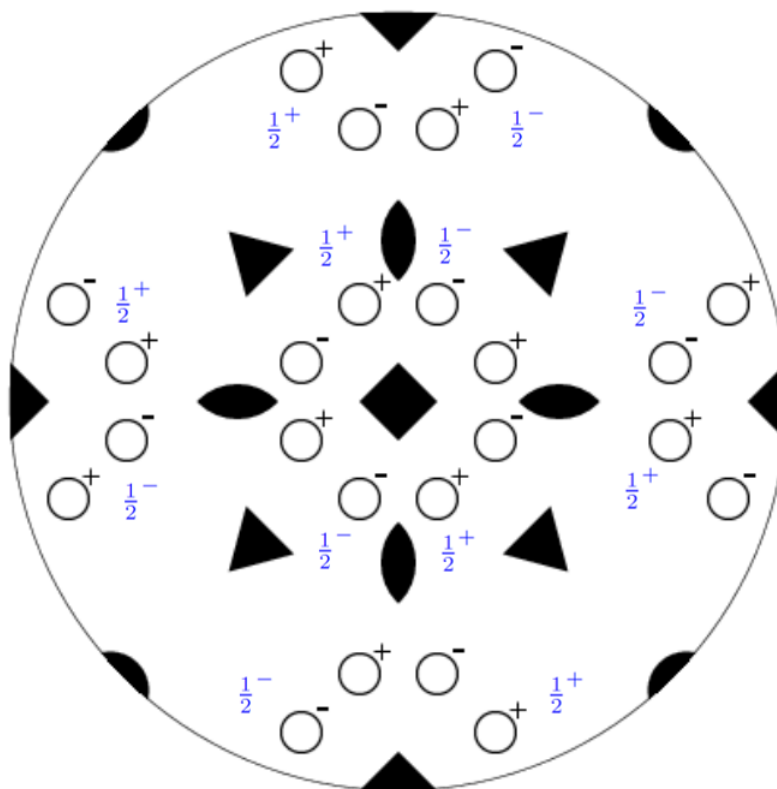



31.1.103

$\bar{4}3m$

$\bar{4}3m$

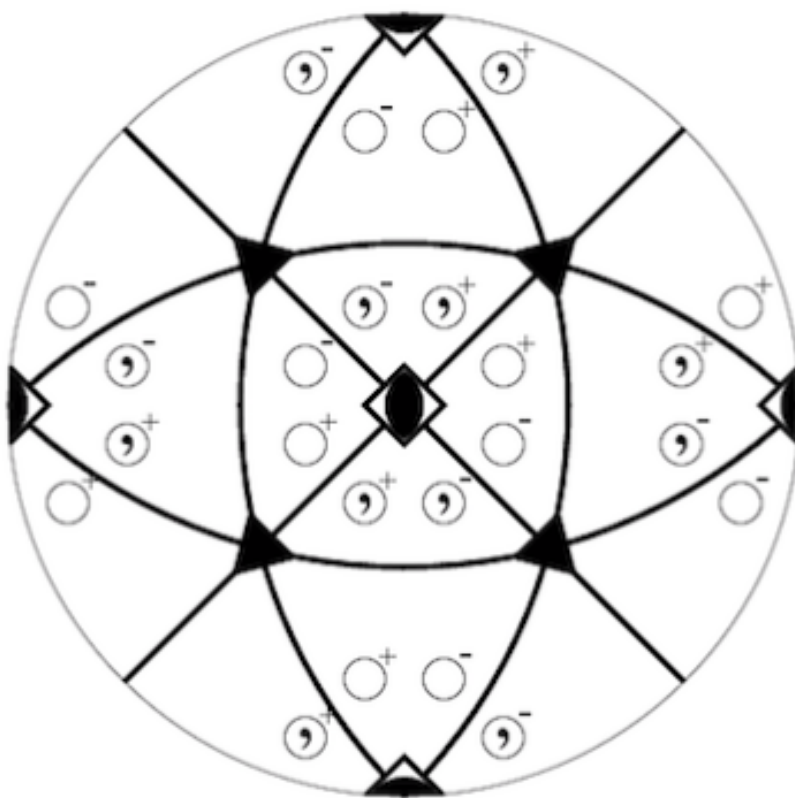

31.2.104

23

$\bar{4}3m$

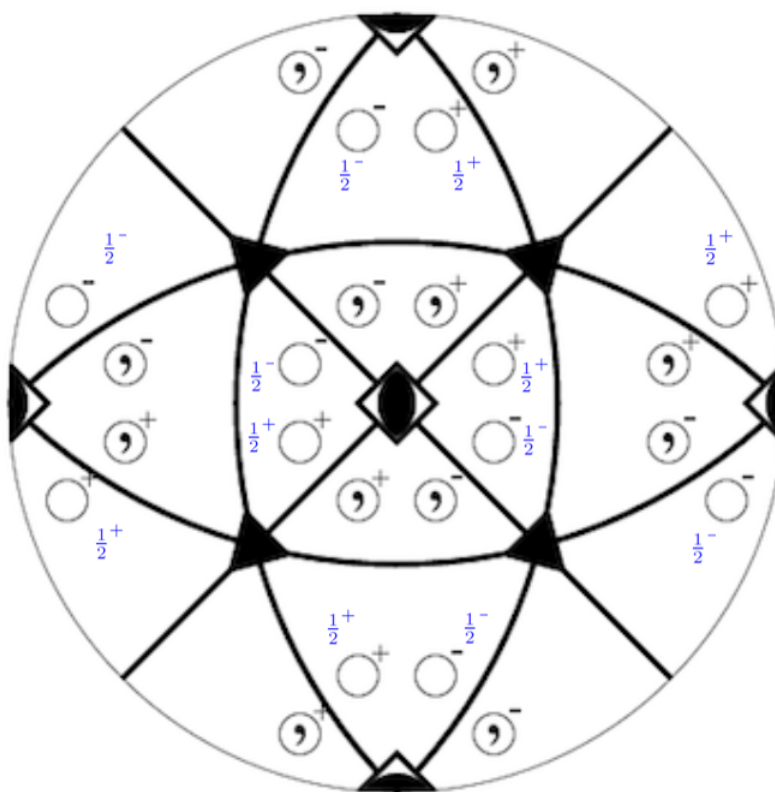

32.1.105

$m\bar{3}m$

$m\bar{3}m$

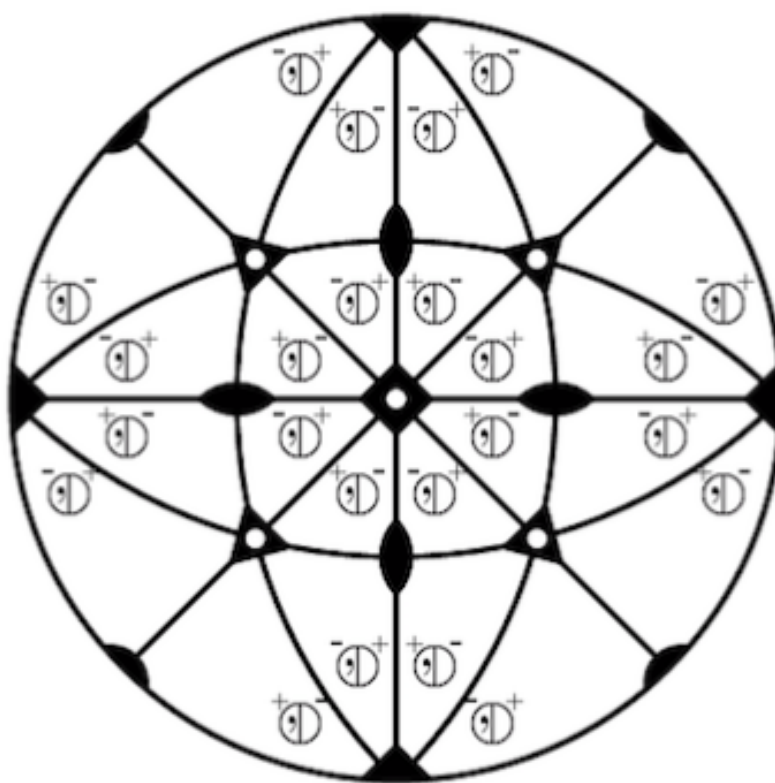

32.2.106

$m\bar{3}$

$m\bar{3}m$

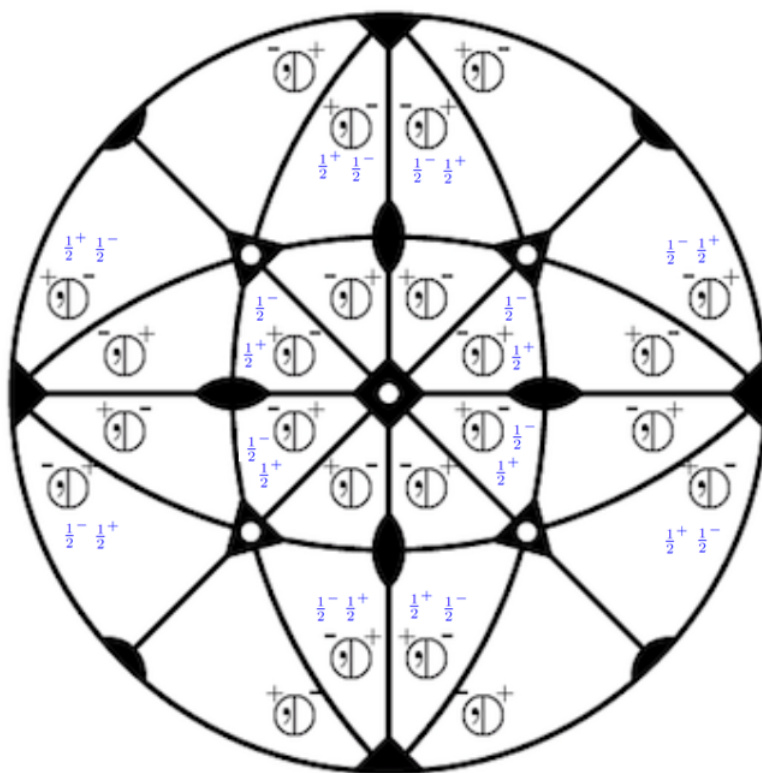

32.3.107

432

$m\bar{3}m$

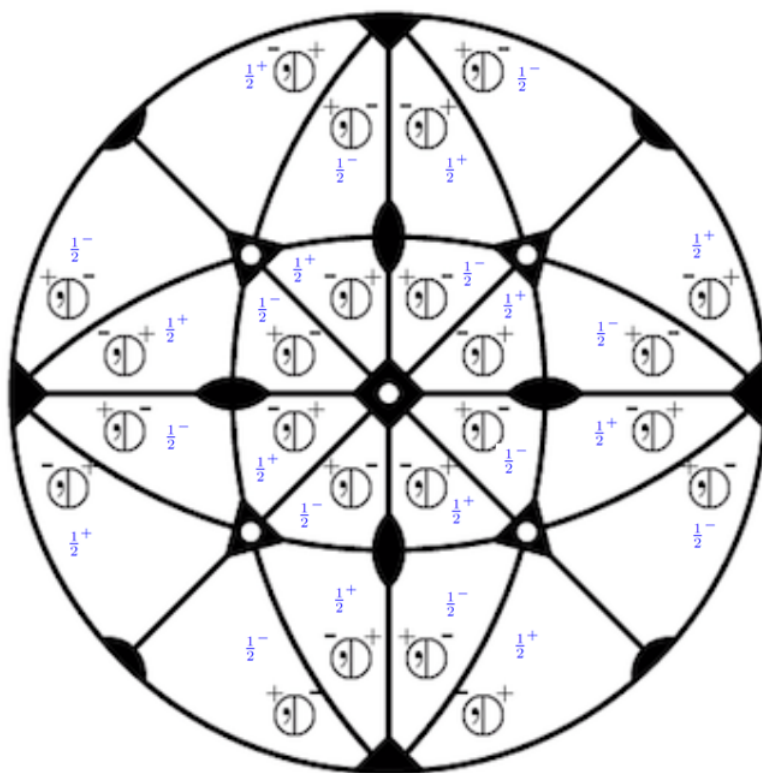

32.4.108

43m

$m\bar{3}m$

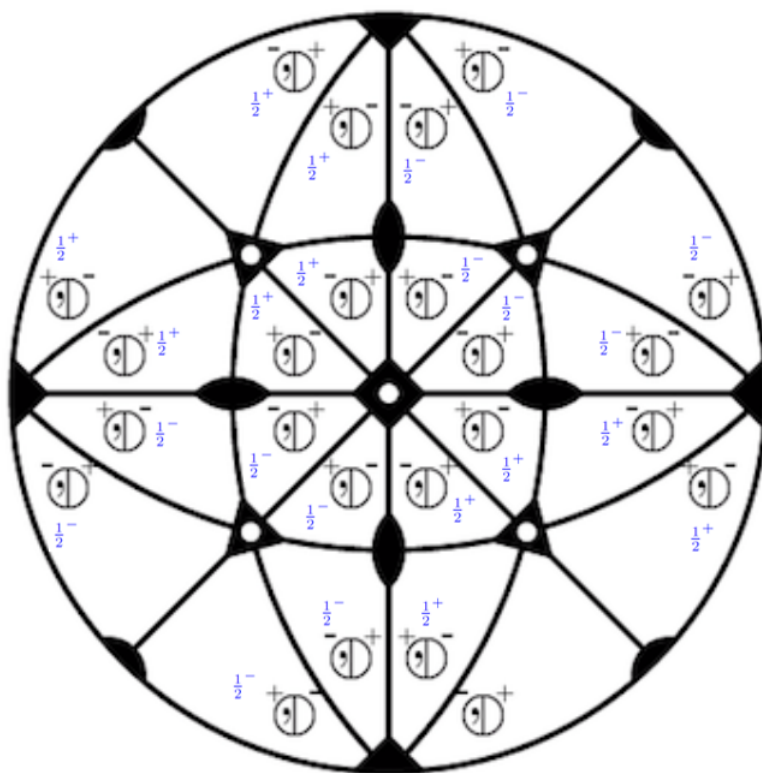

Supplement: Supplementary file 2 [file Stereographic_projections_2.pdf]
